# Supplementary material for: Practical Quasi-Newton Methods for Training Deep Neural Networks
Source: arXiv:2006.08877 source file (2021-01-07)
Supplement: Supplementary file 1 [file 6_lbfgs_implementation.tex]

%\clarify{this section should go to appendix}

If we use LBFGS instead of BFGS \addthis{for $H_g^l$}, as shown in (\ref{eq_1}), we need to compute \deletethis{$H v$} \addthis{$H_g^l v$} where $H_g^l \in R^{d \times d}$ denotes the inverse Hessian induced by LBFGS, and $v = {\mathbf{\nabla f}}_l H^l_a \in R^{d \times d}$. (For simplicity we assume the input and output length are both $d$.)

A naive or vectorized version of two-loop recursion (see Algorithm 7.4 of \cite{nocedal2006numerical}) is far from efficient in this setting. We make use of Theorem 2.2 of \cite{byrd1994representations}. Following the notation in \cite{byrd1994representations},
\begin{align*}
    H 
    & = H_0 + 
    \begin{bmatrix}
        S & H_0 Y
    \end{bmatrix}
    \begin{bmatrix}
        R^{-\top} (D + Y^\top H_0 Y) R^{-1}
        & -R^{-\top}
        \\
        -R^{-1} & 0
    \end{bmatrix}
    \begin{bmatrix}
        S^\top
        \\
        Y^\top H_0
    \end{bmatrix}
    \\
    & = H_0 + 
    \begin{bmatrix}
        S R^{-\top} (D + Y^\top H_0 Y) R^{-1} - H_0 Y R^{-1}
        & - S R^{-\top}
    \end{bmatrix}
    %\begin{bmatrix}
    %    R^{-\top} (D + Y^\top H_0 Y) R^{-1}
    %    & -R^{-\top}
    %    \\
    %    -R^{-1} & 0
    %\end{bmatrix}
    \begin{bmatrix}
        S^\top
        \\
        Y^\top H_0
    \end{bmatrix}
    \\
    & = H_0 + S R^{-\top} (D + Y^\top H_0 Y) R^{-1} S^\top - H_0 Y R^{-1} S^\top - S R^{-\top} Y^\top H_0
    %\begin{bmatrix}
    %    S^\top
    %    \\
    %    Y^\top H_0
    %\end{bmatrix}
    \\
    & = H_0 + \tilde{S} (D + Y^\top H_0 Y) \tilde{S}^\top - H_0 Y \tilde{S}^\top - \tilde{S} Y^\top H_0
    \\
    & \text{(let $\tilde{S} = S R^{-\top}$)}
    %\addthis{
    \\
    &
    = H_0 + 
    \begin{bmatrix}
        \tilde{S} & H_0 Y
    \end{bmatrix}
    \begin{bmatrix}
        D + Y^\top H_0 Y
        & -I
        \\
        -I & 0
    \end{bmatrix}
    \begin{bmatrix}
        \tilde{S}^\top
        \\
        Y^\top H_0
    \end{bmatrix},
    %}
\end{align*}

% \deletethis{
% Hence,
% \begin{align*}
%     H v
%     & = H_0 v + \tilde{S} (D + Y^\top H_0 Y) \tilde{S}^\top v - H_0 Y \tilde{S}^\top v - \tilde{S} Y^\top H_0 v
%     \\
%     & = \gamma v + \tilde{S} (D + \gamma Y^\top Y) \tilde{S}^\top v - \gamma Y \tilde{S}^\top v - \gamma \tilde{S} Y^\top v
%     \\
%     & \text{(let $H_0 = \gamma I$)}
% \end{align*}

% Alternatively, 
% \begin{align*}
%     H 
%     & = H_0 + \tilde{S} (D + Y^\top H_0 Y) \tilde{S}^\top - H_0 Y \tilde{S}^\top - \tilde{S} Y^\top H_0
%     \\
%     & = H_0 + 
%     \begin{bmatrix}
%         \tilde{S} & H_0 Y
%     \end{bmatrix}
%     \begin{bmatrix}
%         D + Y^\top H_0 Y
%         & -I
%         \\
%         -I & 0
%     \end{bmatrix}
%     \begin{bmatrix}
%         \tilde{S}^\top
%         \\
%         Y^\top H_0
%     \end{bmatrix}
% \end{align*}

% Moreover, we can further improve the computational efficiency by updating $R$ and $R^{-1}$ from iteration to iteration. 

% Note that
% }
{where}
\begin{align*}
    R_{i,j} = 
    \begin{cases}
        \vs_{i-1}^\top \vy_{j-1}, & \text{if $i \le j$,}
        \\
        0, & \text{otherwise.}
    \end{cases}
\end{align*}

{Note that we can easily update $R$ from iteration to iteration and then compute $R^{-1}$ by the property of triangular matrices. Alternatively, we can also update $R^{-1}$ from iteration to iteration. Both approaches does not require the inversion operation on a regular matrix. We use the latter one in our experiments. }
