# Supplementary material for: Practical Quasi-Newton Methods for Training Deep Neural Networks
Source: arXiv:2006.08877 source file (2021-01-07)
Supplement: Supplementary file 2 [file conv.tex]

This section derives the Hessian for a convolutional layer. We follows the notation in \cite{grosse2016kronecker}. 

To repeat, the core operation of a convoutional layer (see (12) of \cite{grosse2016kronecker}) is
\begin{align*}
    s_{i,t} = \sum_{\delta} w_{i,j,\delta} a_{j,t+\delta} + b_i,
\end{align*}
where $w$'s are weights, $b$'s is biases, $a$'s are input from last layer, $s$'s are pre-activation of this layer. In terms of indices, $i$ denotes the output channel, $j$ denotes the input channel, $\delta$ denotes the spatial location in the filter, $t$ denote the spatial location in input/output. 

We first derive the gradient (see (13) of \cite{grosse2016kronecker}). We use $E$ to denote the loss. Then,
\begin{align*}
    \frac{\partial E}{\partial w_{i,j,\delta}}
    = \sum_t \frac{\partial E}{\partial s_{i,t}} \frac{\partial s_{i,t}}{\partial w_{i,j,\delta}}
    = \sum_t \frac{\partial E}{\partial s_{i,t}} a_{j,t+\delta}
\end{align*}

We then derive the Hessian. We have that
\begin{align*}
    \frac{\partial^2 E}{\partial w_{i,j,\delta} \partial w_{i',j',\delta'}}
    & = \frac{\partial}{\partial w_{i',j',\delta'}} \left( \sum_t \frac{\partial E}{\partial s_{i,t}} a_{j,t+\delta} \right)
    = \sum_t a_{j,t+\delta} \frac{\partial}{\partial w_{i',j',\delta'}} \left( \frac{\partial E}{\partial s_{i,t}} \right)
    \\
    & = \sum_t a_{j,t+\delta} \sum_{t'} \frac{\partial}{\partial s_{i',t'}} \left( \frac{\partial E}{\partial s_{i,t}} \right) \frac{\partial s_{i',t'}}{\partial w_{i',j',\delta'}}
    \\
    & = \sum_t a_{j,t+\delta} \sum_{t'} \frac{\partial}{\partial s_{i',t'}} \left( \frac{\partial E}{\partial s_{i,t}} \right) a_{j', t'+\delta'}
    \\
    & = \sum_{t,t'} a_{j,t+\delta} a_{j', t'+\delta'} \frac{\partial^2 E}{\partial s_{i,t} \partial s_{i',t'}}
\end{align*}

Note that the Hessian matrix is $\frac{\partial^2 E}{\partial \text{vec}(w) \partial \text{vec}(w)}$. We first focus on one block of it, where $j, \delta, j', \delta'$ is fixed. This block is
\begin{align*}
    \sum_{t,t'} a_{j,t+\delta} a_{j', t'+\delta'} B_{t,t'}
\end{align*}
where $B_{t,t'} = \left( \frac{\partial^2 E}{\partial s_{i,t} \partial s_{i',t'}} \right)_{i,i'}$. We further define $A_{t, t'} = \left( a_{j,t+\delta} a_{j', t'+\delta'} \right)_{j, j', \delta, \delta'}$. (Note that the valid indices $t, t'$ should be w.r.t $s$.) Then,
\begin{align*}
    \frac{\partial^2 E}{\partial \text{vec}(w) \partial \text{vec}(w)}
    = \sum_{t,t'} A_{t, t'} \otimes B_{t, t'}
\end{align*}

\subsection{Following KFAC's assumptions}

In order to further simplify the expression of Hessian, we first make Assumption \ref{assumption_1}. Note that Assumption \ref{assumption_1} is "equivalent" to the spatially uncorrelated derivatives (SUD) assumption plus (22) of spatial homogeneity (SH) assumption of \cite{grosse2016kronecker}. 
\begin{assumption}
\label{assumption_1}
$B_{t,t'} = 0$ when $t \neq t'$. 
\end{assumption}

By Assumption \ref{assumption_1},
\begin{align*}
    \frac{\partial^2 E}{\partial \text{vec}(w) \partial \text{vec}(w)}
    = \sum_{t} A_{t, t} \otimes B_{t, t}
\end{align*}

We then make Assumption \ref{assumption_2}. Note that Assumption \ref{assumption_2} is "equivalent" to (21) and (22) of SH assumption of \cite{grosse2016kronecker}. 
\begin{assumption}
\label{assumption_2}
Both $A_{t,t}$ and $B_{t,t}$ are independent of $t$. 
\end{assumption}

By Assumption \ref{assumption_2},
\begin{align*}
    \frac{\partial^2 E}{\partial \text{vec}(w) \partial \text{vec}(w)}
    & = |T| \left( A_{t_0, t_0} \otimes B_{t_0, t_0} \right)
    = |T| \left( \frac{1}{|T|} \sum_t A_{t, t} \right) \otimes \left( \frac{1}{|T|} \sum_t B_{t, t} \right)
    \\
    & = \frac{1}{|T|} \left( \sum_t A_{t, t} \right) \otimes \left(  \sum_t B_{t, t} \right)
\end{align*}

Finally, in order to use K-BFGS, we can easily compute $\sum_t A_{t, t}$, and do BFGS update on $\sum_t B_{t, t}$. 

\subsubsection{An alternative to (32) of \texorpdfstring{\cite{grosse2016kronecker}}{TEXT}}

%Note that for simplicity, we focus on a single data point. 
To make things as simple as possible, consider the case of a single data point with only one input channel (i.e. $J = 1$) and a 1-d convolutional layer. 

The first equation of (32) of \cite{grosse2016kronecker} gives a way of computing $\sum_t A_{t,t}$. Note that
$
    \sum_t A_{t,t}
    = \sum_t \left( a_{j,t+\delta} a_{j', t+\delta'} \right)_{j, j', \delta, \delta'}
$
. The complexity of computing each individual matrix is $O(J^2 |\Delta|^2)$. Hence, the total complexity is $O(J^2 |\Delta|^2 |T|)$. 

We propose an alternative approach to the above naive way of computing $\sum_t A_{t,t}$. In particular, we first compute $\sum_t \left( a_{j,t+\delta} a_{j', t+\delta'} \right)_{j, j'}$ for fixed $\delta$, $\delta'$. Because we are looking at the case of 1-d convolutional layer, $\delta, \delta' \in R$. Furthermore, because $J = 1$,
\begin{align}
    \sum_t \left( a_{j,t+\delta} a_{j', t+\delta'} \right)_{j, j'}
    = \sum_t a_{1,t+\delta} a_{1, t+\delta'}
    \label{eq_2}
\end{align}
The key to our new approach is to notice that, in the above summation, the "major" part remains unchanged if $\delta - \delta'$ is the same. For example, when $(\delta, \delta') = (0, 1)$ and $(\delta, \delta') = (1, 2)$, the "major" part in the summation of the RHS of (\ref{eq_2}) is the same. Hence, we can compute multiple $(\delta, \delta')$ pairs at the same time with minimal overhead. 

Note that $d_{\delta} = \delta - \delta' \in \{ -|\Delta|, \cdots, |\Delta| \}$. For a given $d_{\delta}$, we first compute $a_{1, t} a_{1, t + d_{\delta}}$ for all $t$ such that $t, t + d_{\delta} \in \mathcal{T}$, resulting in $O(|T|)$ complexity. Then, we can compute $\sum_t a_{1,t+\delta} a_{1, t+\delta'}$ for all $\delta$, $\delta'$ such that $\delta - \delta' = d_{\delta}$, by summing up the needed part, resulting in $O(|\Delta| |T|)$. 

%\subsection{Another set of assumptions}
