# Supplementary material for: Practical Quasi-Newton Methods for Training Deep Neural Networks
Source: arXiv:2006.08877 source file (2021-01-07)
Supplement: Supplementary file 3 [file empirical_justification.tex]

\section{
{Empirical justification of K-BFGS approximation}
}
\label{sec_7}

\clarify{
- have a color bar for all three figures; have another set of figs with gray color (I'm not 100\% clear for this part TBH...)

- see why scale of Hessian is larger at initial layers

- compute block Hessian based on the whole dataset
}

The Kronecker block-wise approximation to the Hessian leads to significant computational savings
in terms of storage and inversion, which allowed us to to design an efficient algorithm for computing an approximation to the inverse Hessian. In this section, we explore numerically, through a toy example, the validity of our approximations.

We consider the fully connected neural network with the following architecture 256-20-20-20-20-10 with standard tanh units and no bias terms. We train the neural network to classify a down-scaled 16x16 version of MNIST dataset. We trained the network with 10 epochs of K-BFGS with batch size equal to 1000 achieving 6 \% training error. We then computed the actual Full-Hessian over a mini-batch of size 1000 and compared it to our K-BFGS approximation.

\subsection{Block diagonal structure}

We first examine the structure of the exact hessian of the middle 4 layers of the network in Figure \ref{fig:kron_approx}.
\begin{figure}[H]
\begin{centering}

\includegraphics[width=.25\columnwidth]{figures/loghessian/logscaledhessian.png}
\hspace{0.025\columnwidth}
\includegraphics[width=.25\columnwidth]{figures/loghessian/blockwiseL1.png}
\hspace{0.025\columnwidth}
\includegraphics[width=.25\columnwidth]{figures/loghessian/logscaledkhessian.png}

\caption{\small A comparison of the exact hessian and our block-wise Kronecker-factored BFGS approximation, for the middle 4 layers.  On the \textbf{left} is the exact absolute values of the Hessian, in the \textbf{middle} is the block wise frobenius norm of the true Hessian, and on the \textbf{right} is the K-BFGS approximation. Note that for the purposes of visibility we plot the absolute values of the entries, with the white level corresponding linearly to the size of these values (up to some maximum for each image). \label{fig:kron_approx} }
\end{centering}
\end{figure}

\clarify{(Need to add comments on this part.)}

\subsection{Diagonal block-wise comparison}

\clarify{Are we still including this part? -Yi}

% \clarify{need to replace the minibatch with the whole data set in the left column of Figure \ref{fig:kron_approx_blocks}}

% \begin{figure}[h]

% \begin{centering}

% \includegraphics[width=.25\columnwidth]{figures/numhessian/block11h.png}
% \hspace{0.025\columnwidth}
% \includegraphics[width=.25\columnwidth]{figures/numhessian/block11kbfgs.png}

% \vspace{0.025\columnwidth}
% \includegraphics[width=.25\columnwidth]{figures/numhessian/block22h.png}
% \hspace{0.025\columnwidth}
% \includegraphics[width=.25\columnwidth]{figures/numhessian/block22kbfgs.png}

% \vspace{0.025\columnwidth}
% \includegraphics[width=.25\columnwidth]{figures/numhessian/block33h.png}
% \hspace{0.025\columnwidth}
% \includegraphics[width=.25\columnwidth]{figures/numhessian/block33kbfgs.png}

% \vspace{0.025\columnwidth}
% \includegraphics[width=.25\columnwidth]{figures/numhessian/block44h.png}
% \hspace{0.025\columnwidth}
% \includegraphics[width=.25\columnwidth]{figures/numhessian/block44kbfgs.png}

% \caption{\small A comparison of the exact hessian and our block-wise Kronecker-factored BFGS approximation, for the middle 4 layers.  The column on the \textbf{left} are the diagonal blocks of the exact absolute values of the Hessian, and on the \textbf{right} is the K-BFGS approximation. Note that for the purposes of visibility we plot the absolute values of the entries, with the white level corresponding linearly to the size of these values (up to some maximum for each image). \label{fig:kron_approx_blocks} }
% \end{centering}
% \end{figure}
