# Supplementary material for: Practical Quasi-Newton Methods for Training Deep Neural Networks
Source: arXiv:2006.08877 source file (2021-01-07)
Supplement: Supplementary file 4 [file experiment_not_used.tex]

Fig \ref{fig_1}, \ref{fig_2}, \ref{fig_3}:

\begin{figure}[ht]
  \centering
  \includegraphics[width=\textwidth]{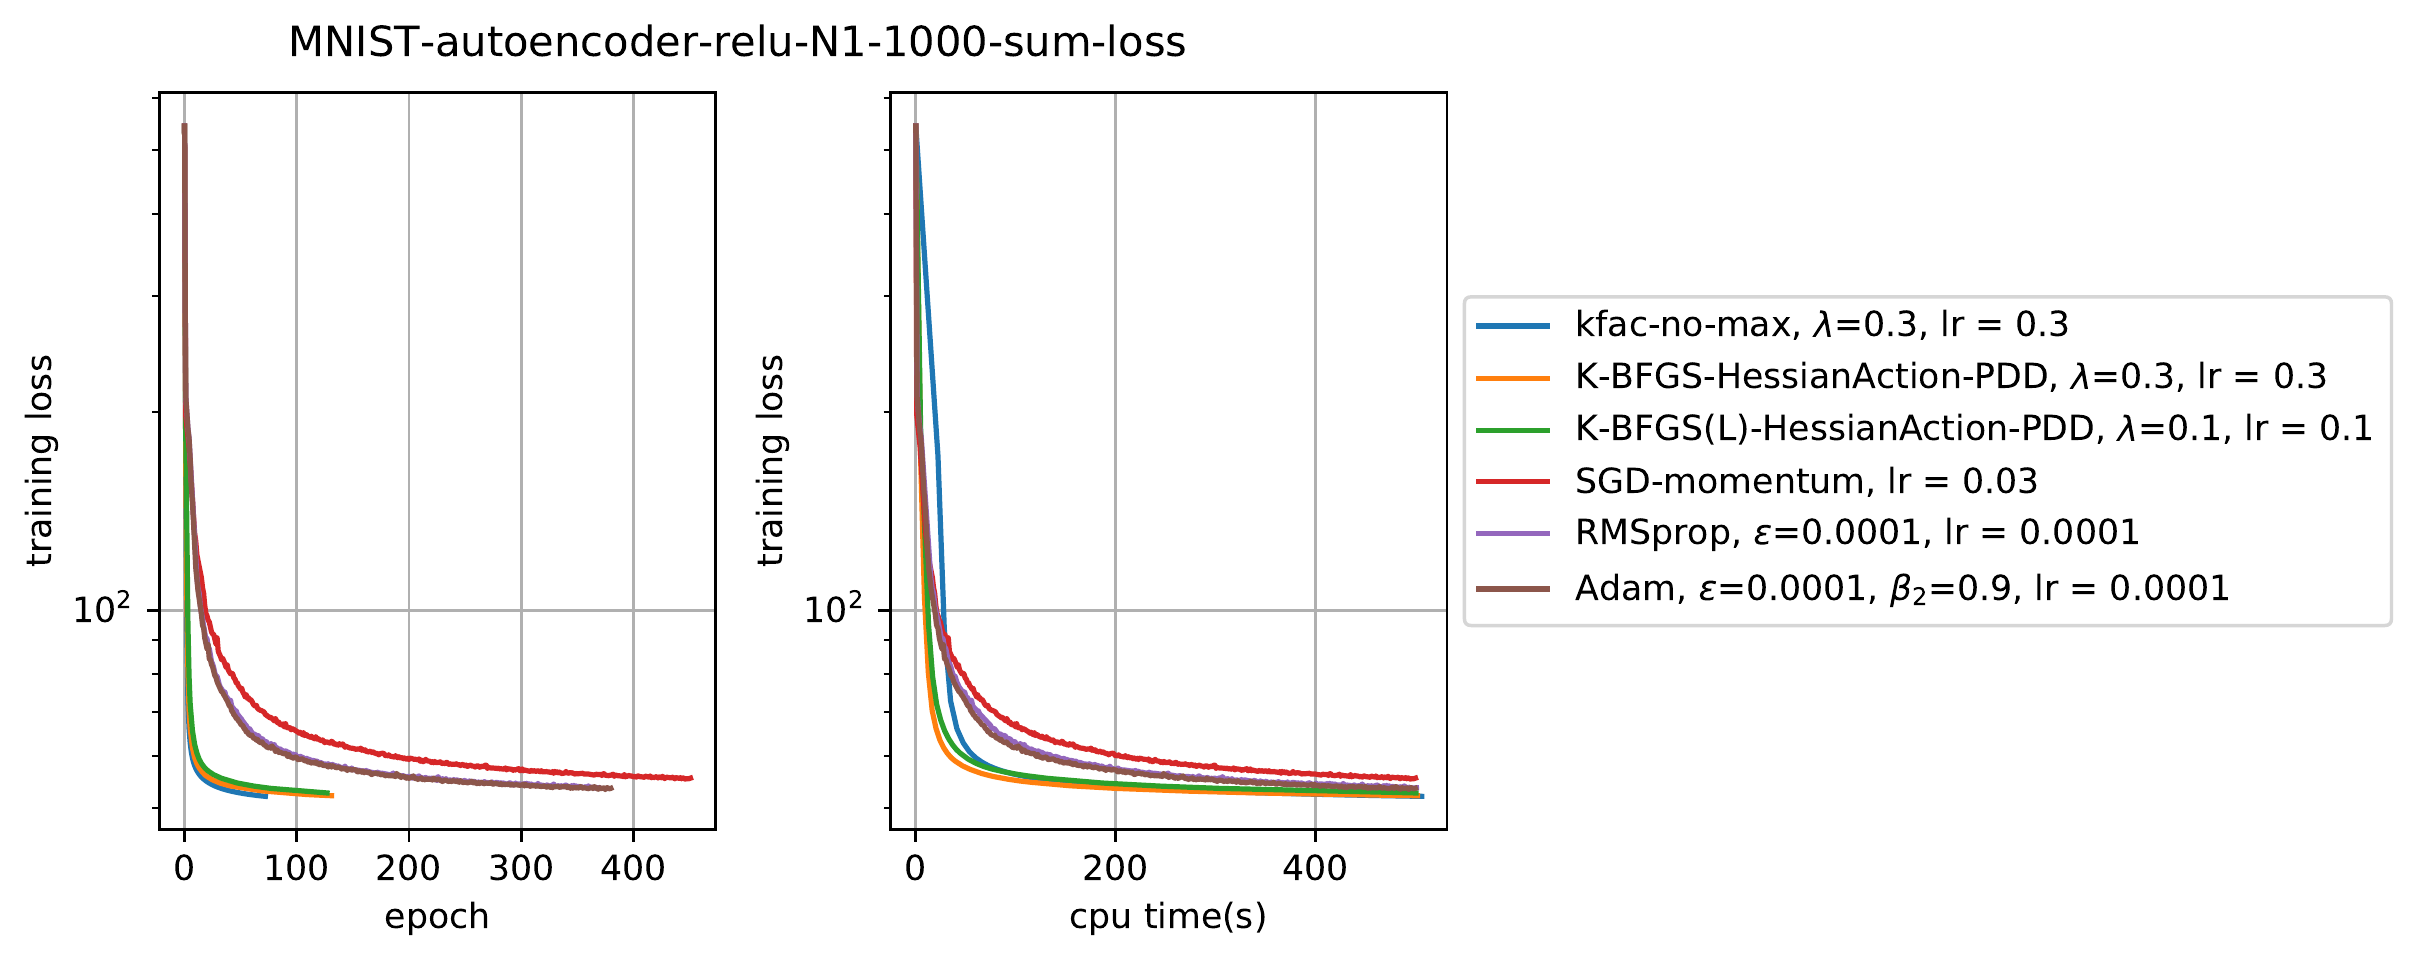}
  \caption{MNIST}
  \label{fig_1}
\end{figure}

\begin{figure}[ht]
  \centering
  \includegraphics[width=\textwidth]{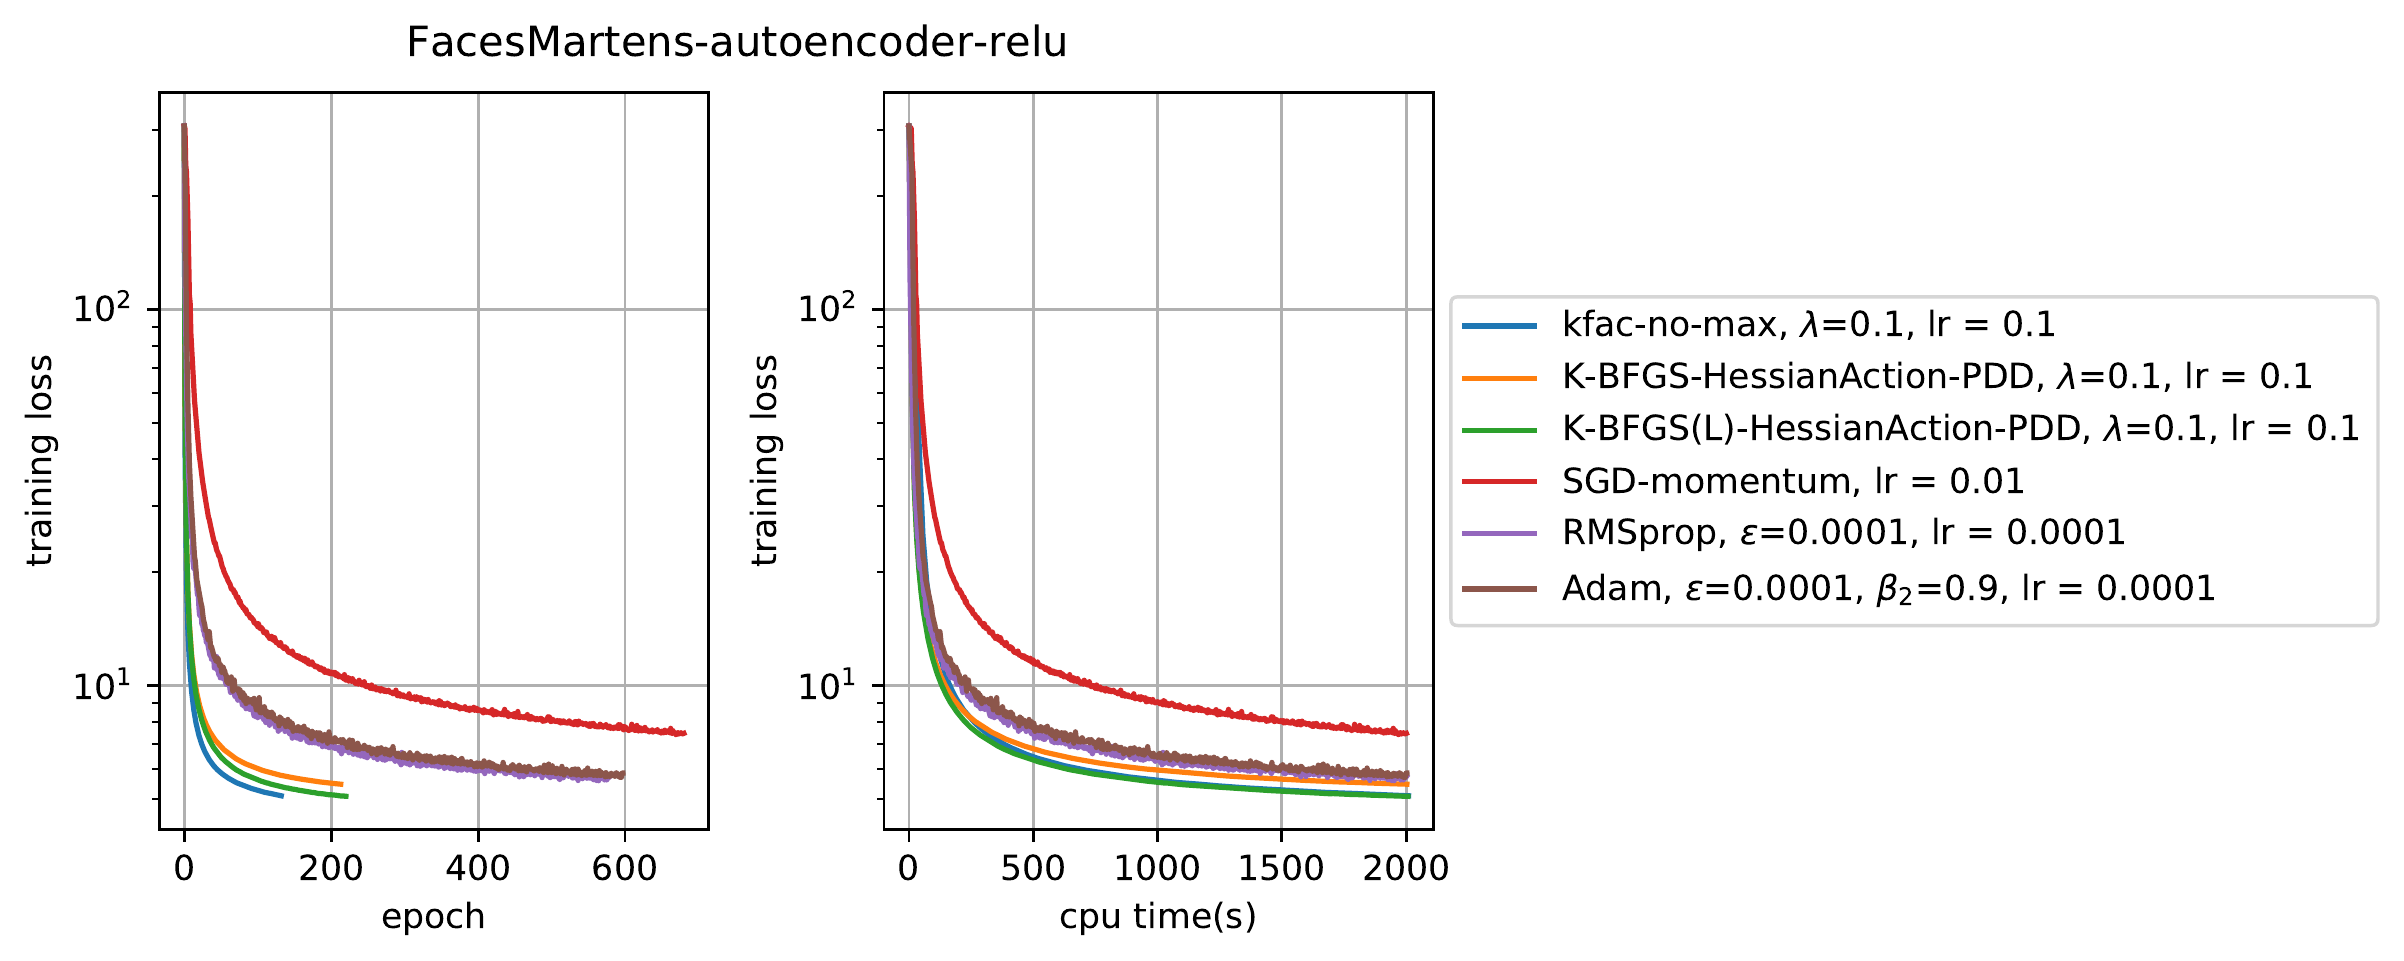}
  \caption{FACES}
  \label{fig_2}
\end{figure}

\begin{figure}[ht]
  \centering
  \includegraphics[width=\textwidth]{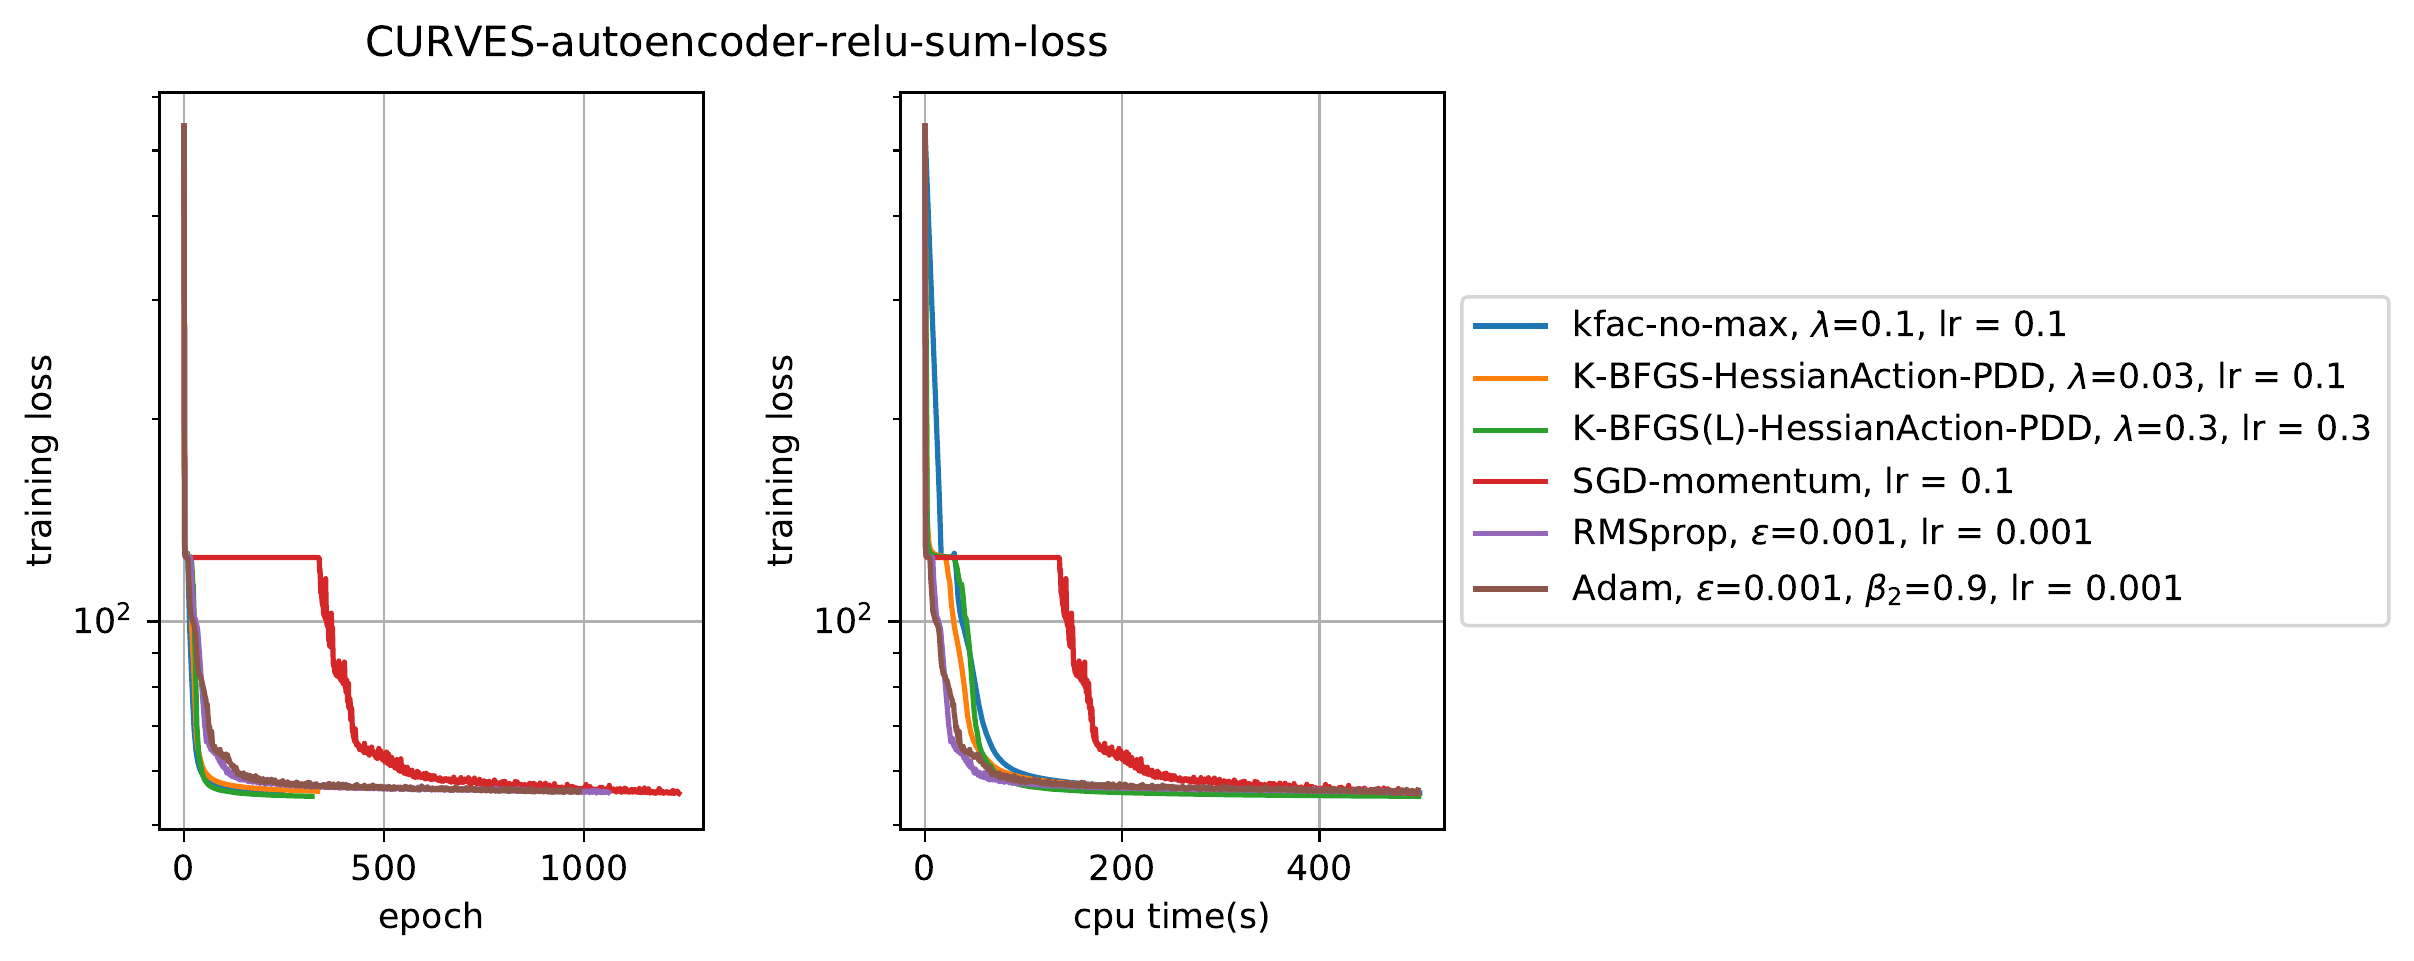}
  \caption{CURVES}
  \label{fig_3}
\end{figure}

% \begin{figure}[ht]
% \begin{centering}
%     \includegraphics[width=\columnwidth]{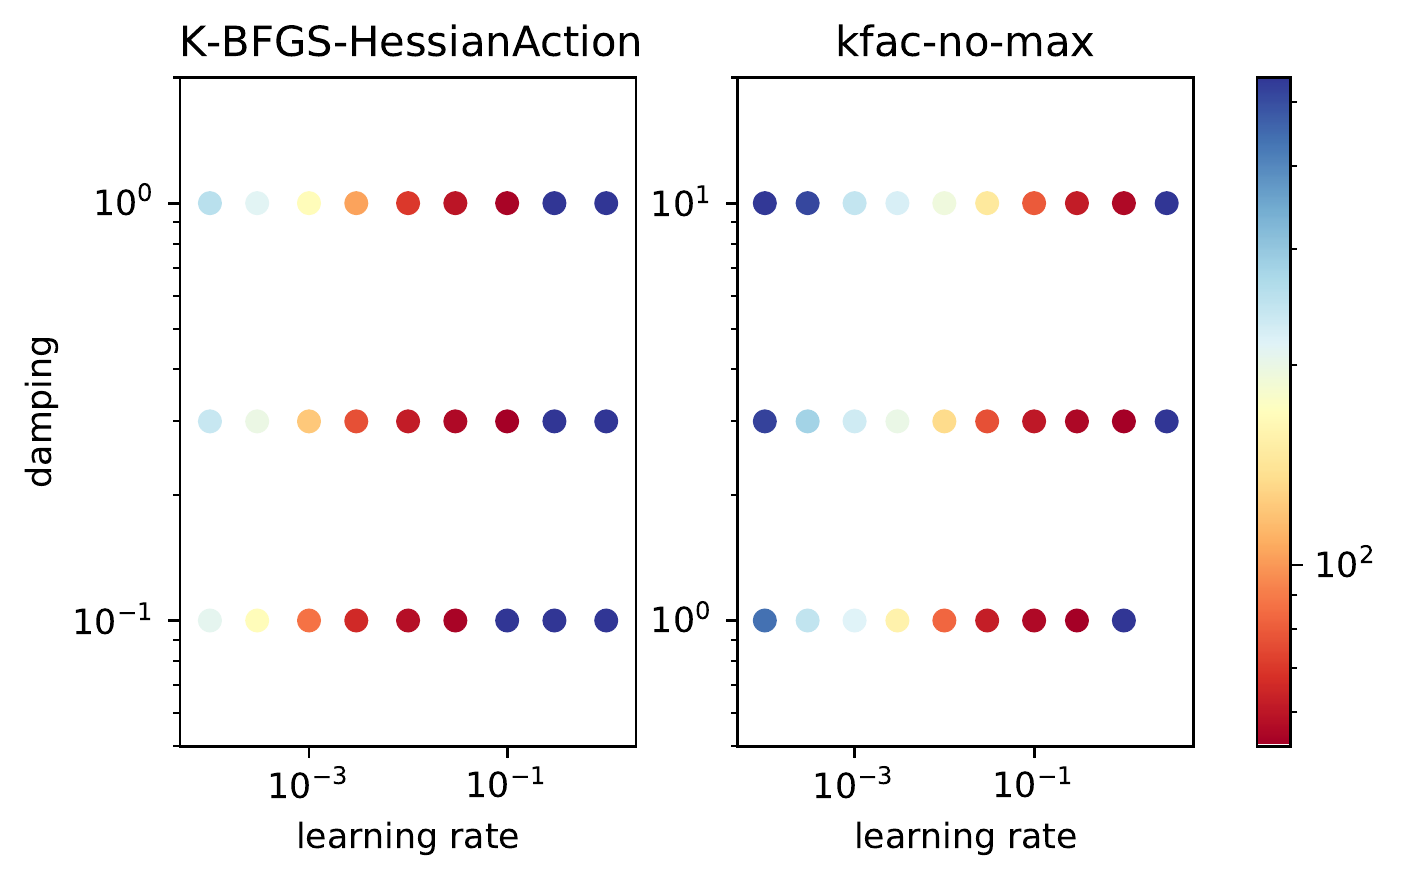}
%     \caption{MNIST, after 500 seconds (process time)}
%     \label{fig_5}
% \end{centering}
% \end{figure}

% \begin{figure}[ht]
% \begin{centering}
%     \includegraphics[width=\columnwidth]{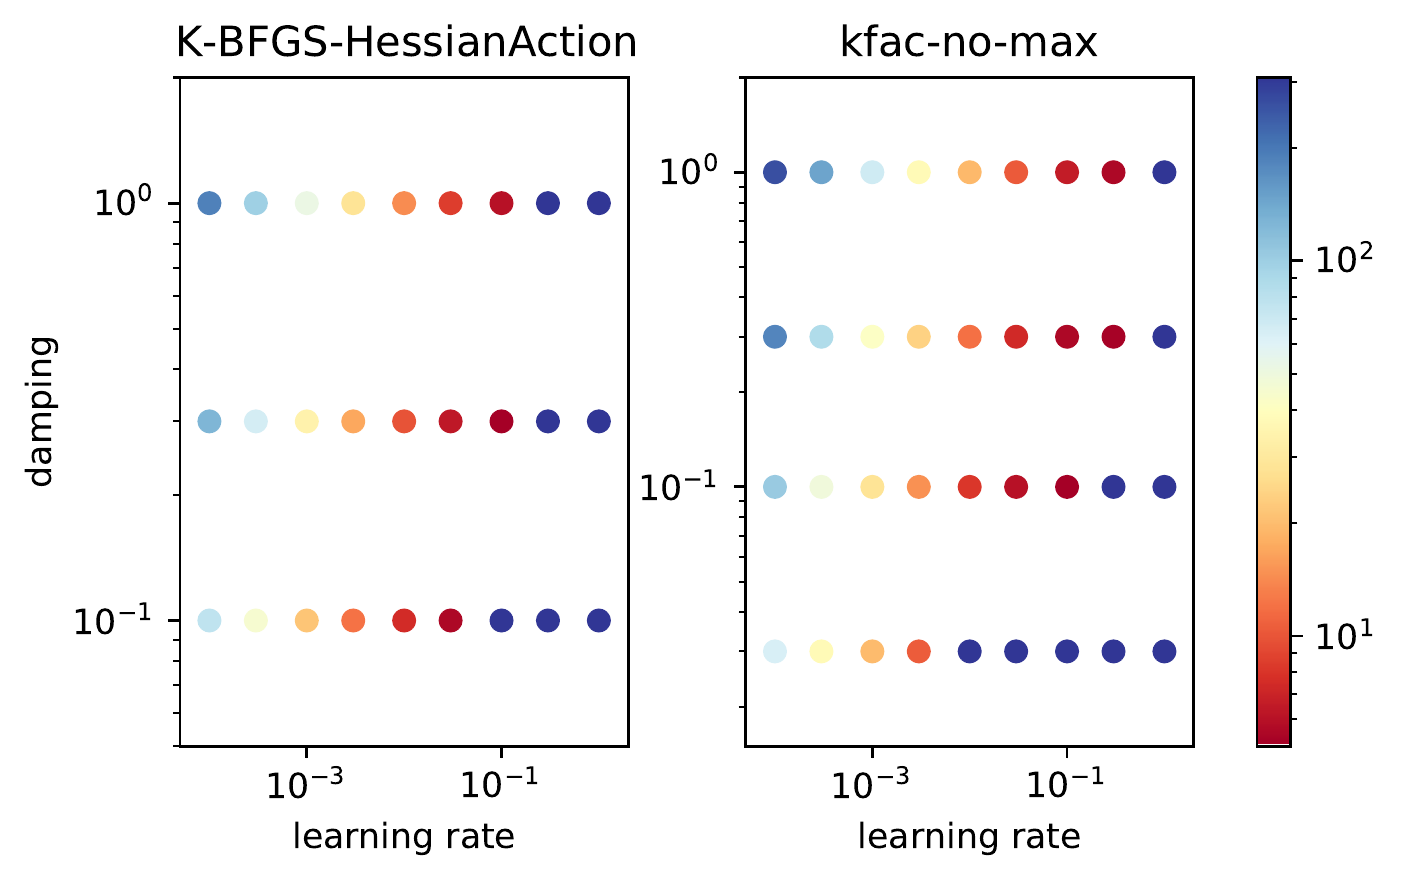}
%     \caption{FACES, after 2000 seconds (process time)}
%     \label{fig_6}
% \end{centering}
% \end{figure}

% \begin{figure}[ht]
% \begin{centering}
%     \includegraphics[width=\columnwidth]{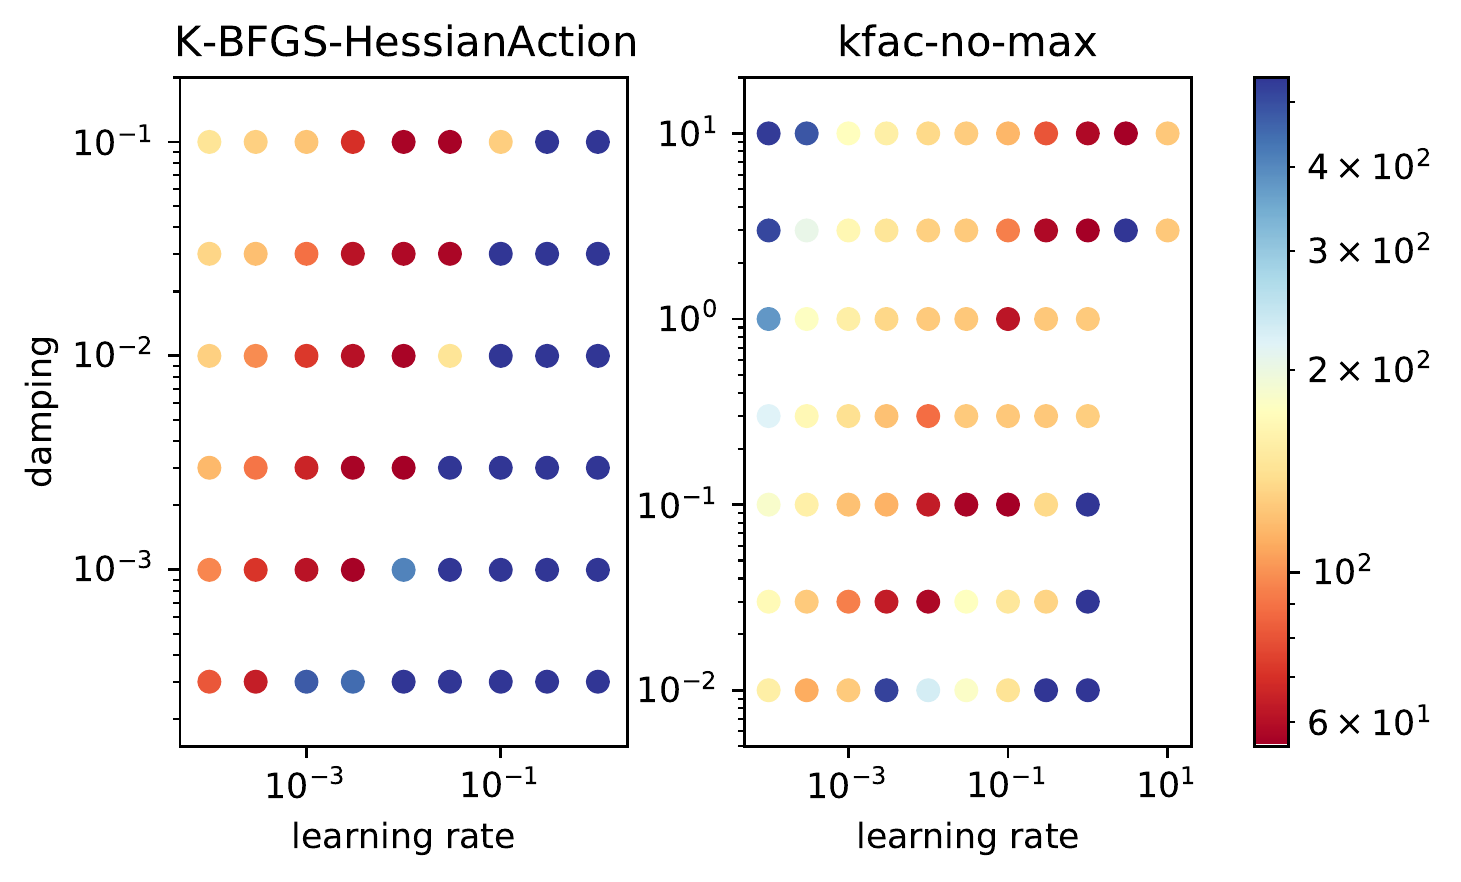}
%     \caption{CURVES, after 500 seconds (process time)}
%     \label{fig_7}
% \end{centering}
% \end{figure}

Figure \ref{fig_11}:

\begin{figure}[ht]
\centering

\begin{minipage}{.33\textwidth}
  \centering
  \includegraphics[width=\textwidth]{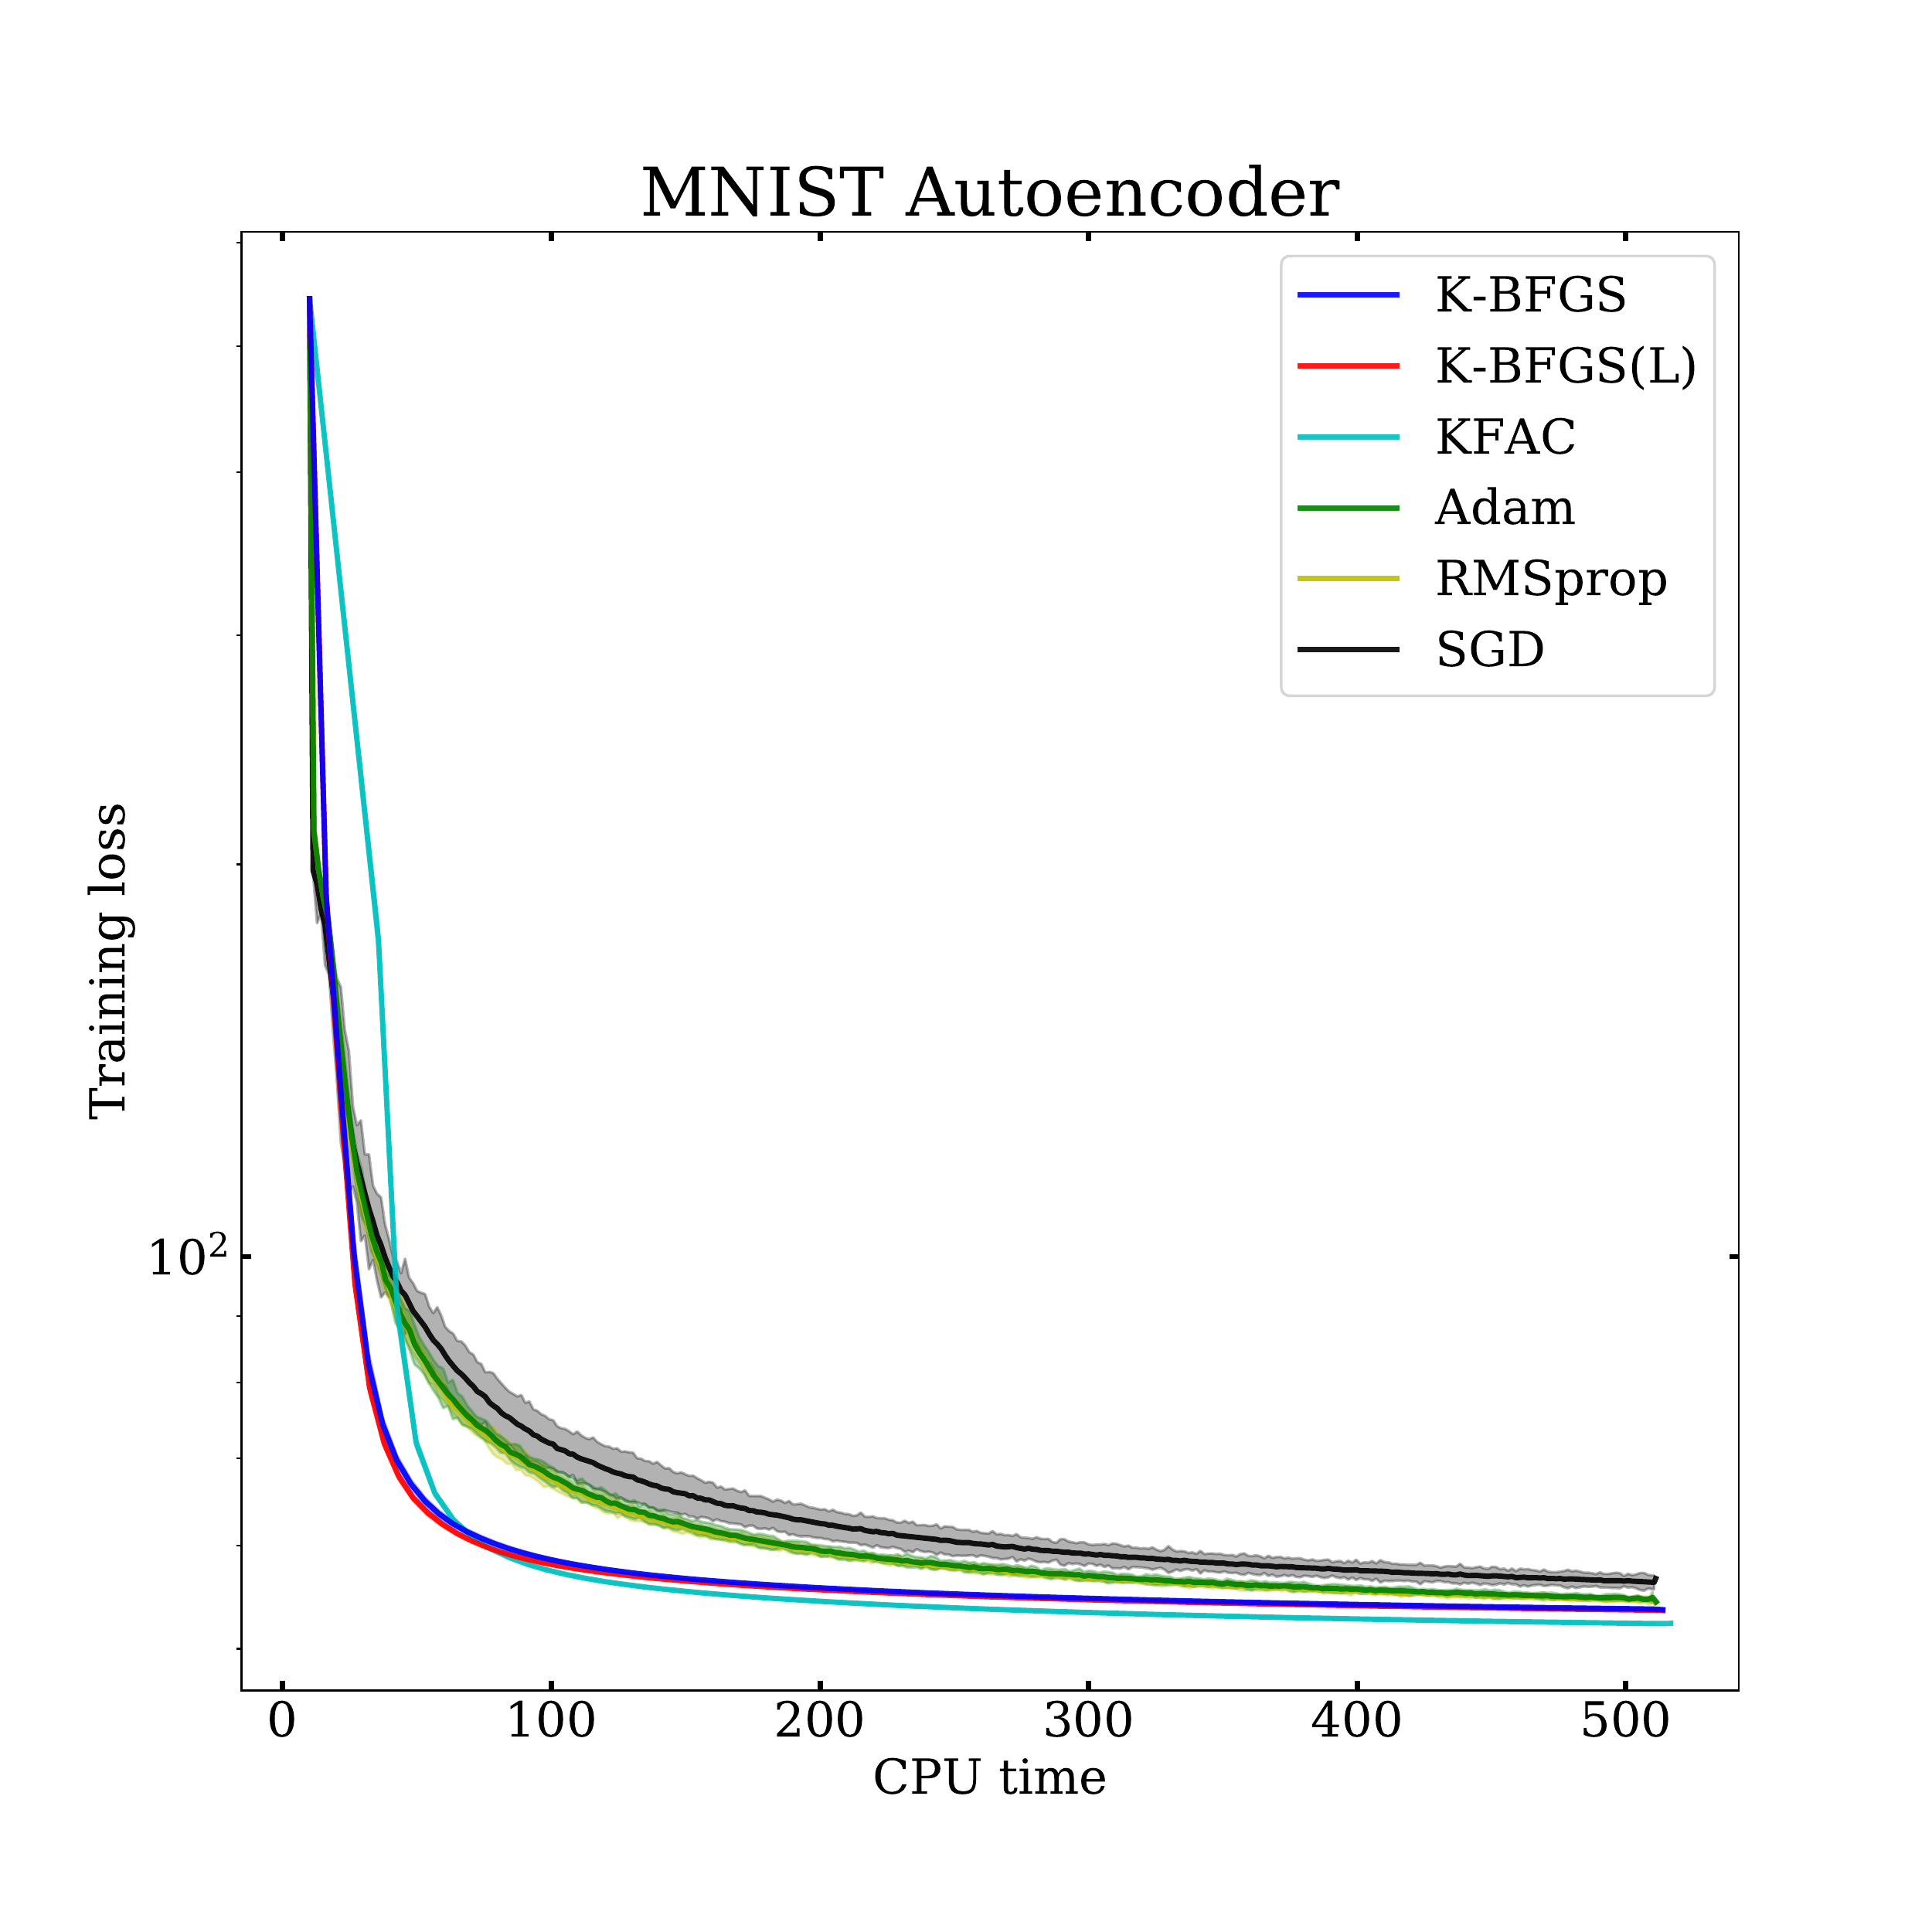}
\end{minipage}%
\begin{minipage}{.33\textwidth}
  \centering
  \includegraphics[width=\textwidth]{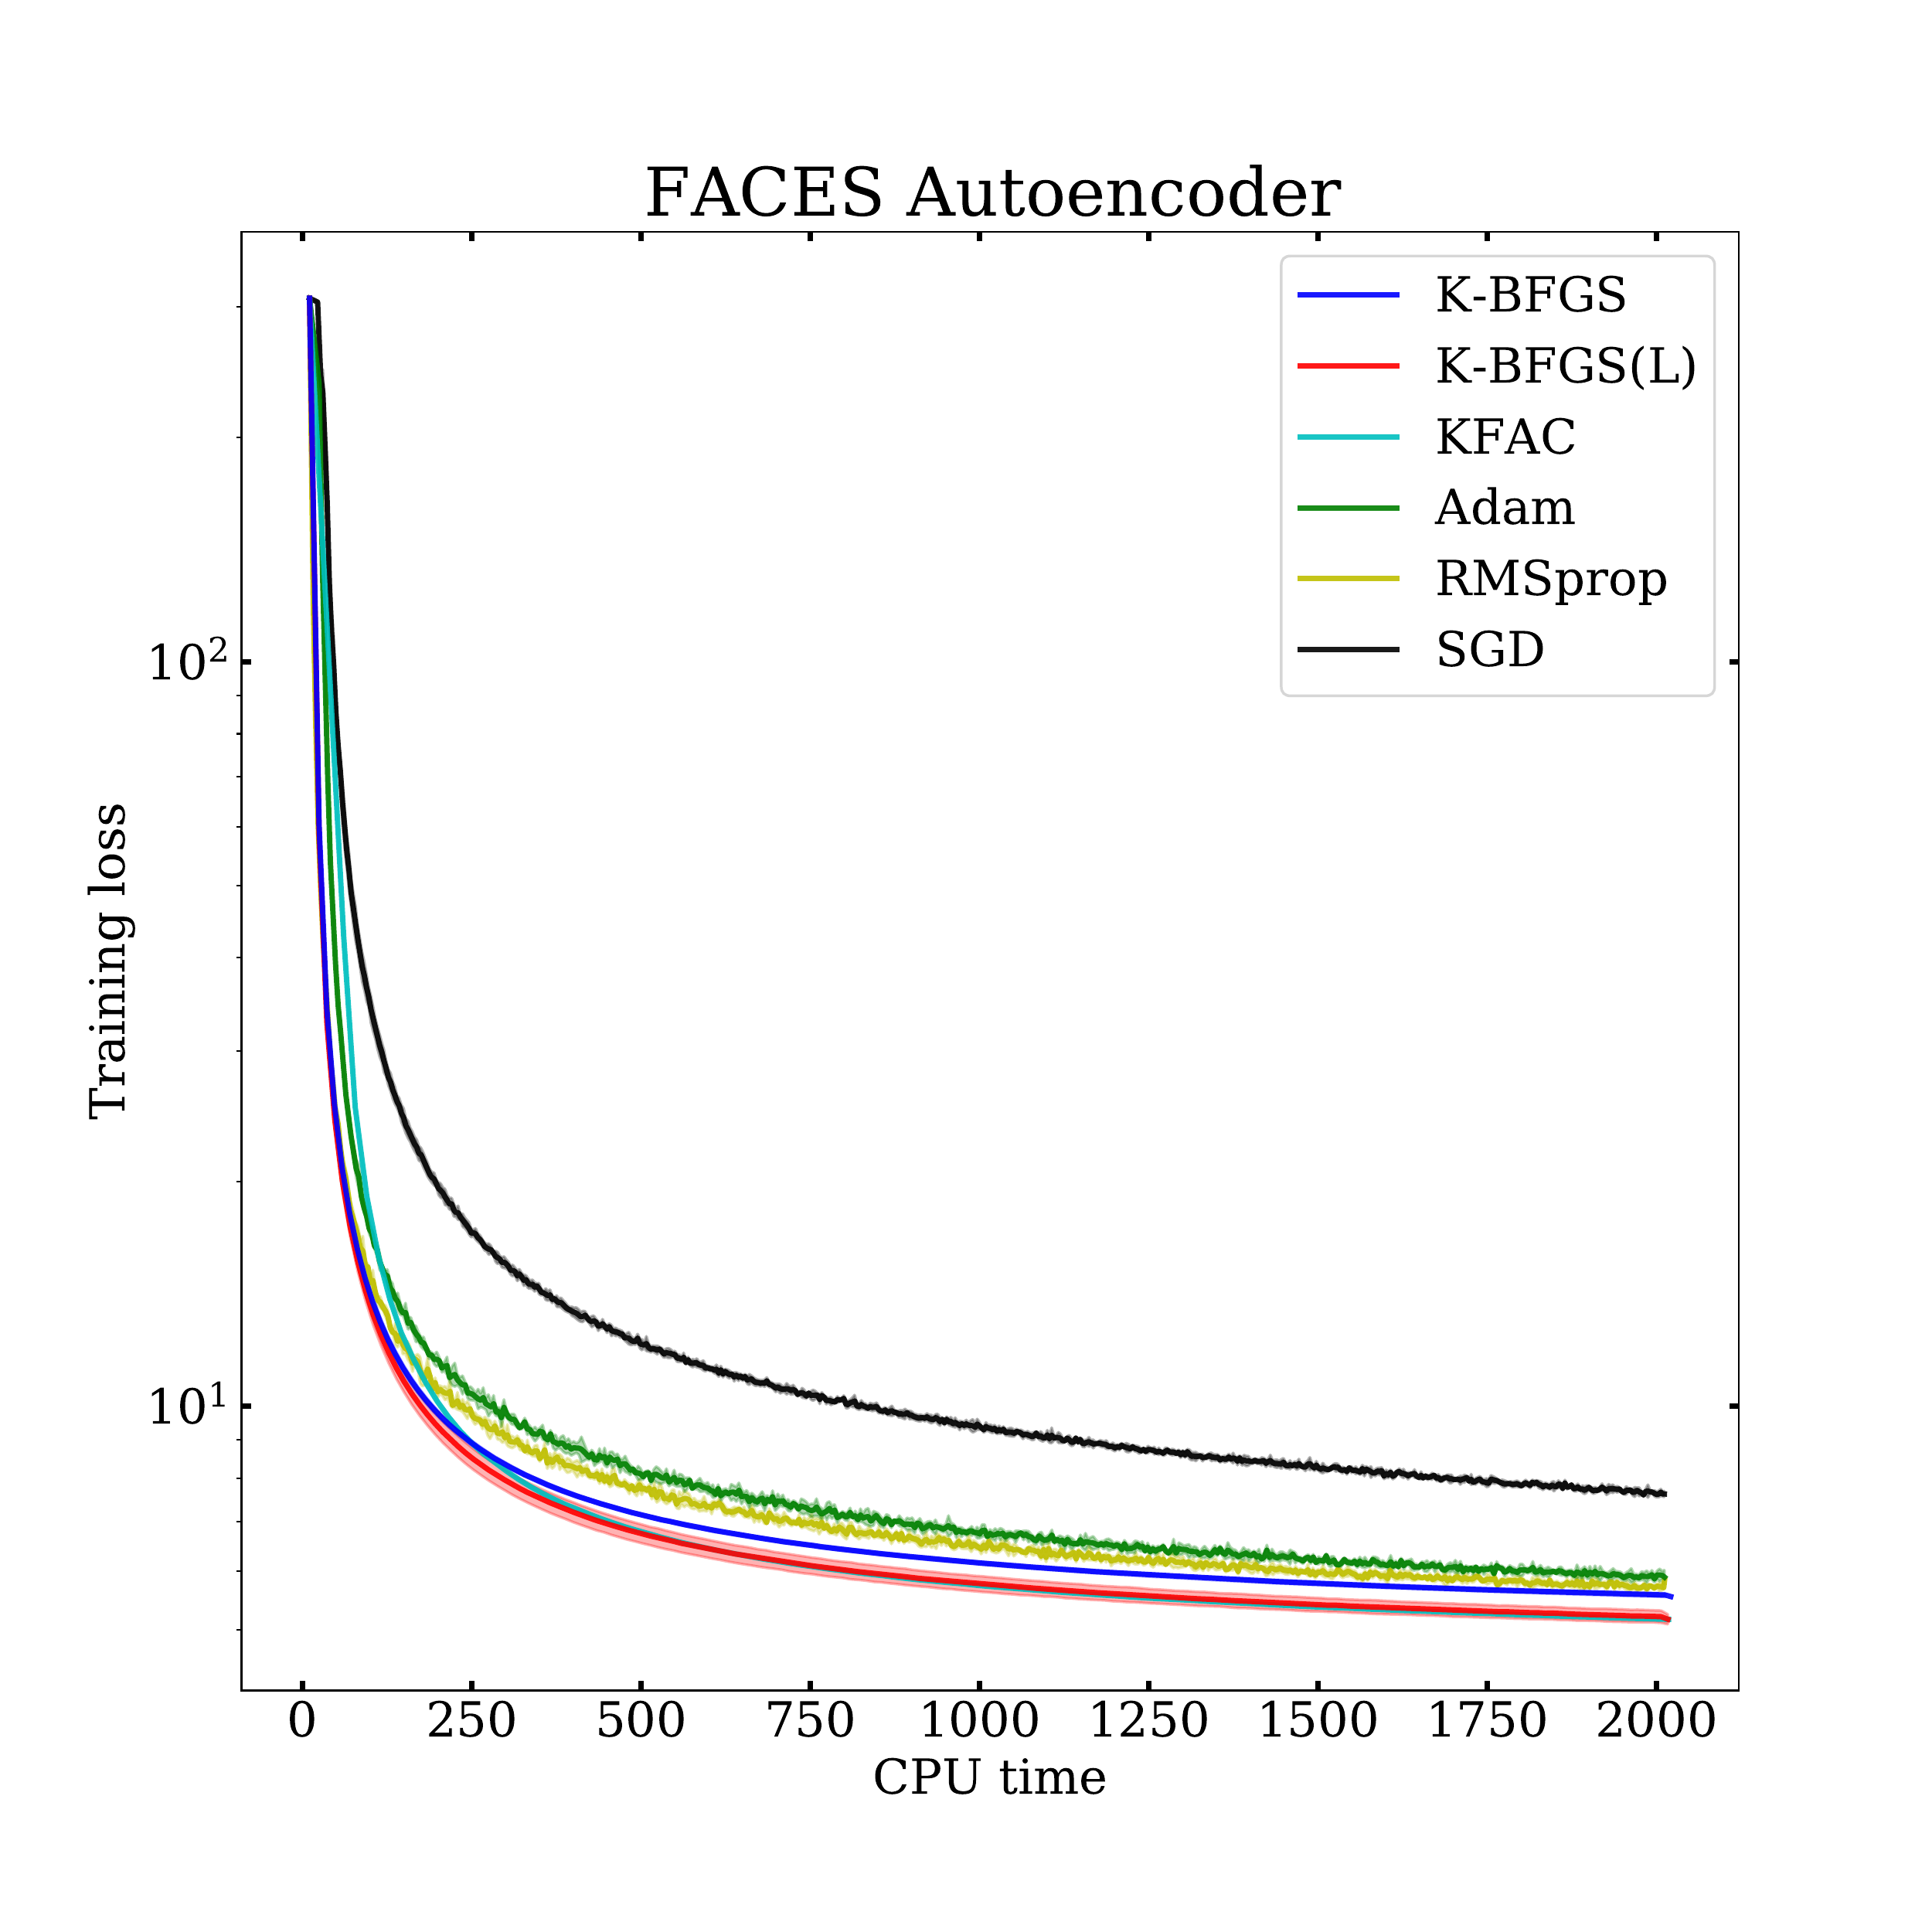}
\end{minipage}%
\begin{minipage}{.33\textwidth}
  \centering
  \includegraphics[width=\textwidth]{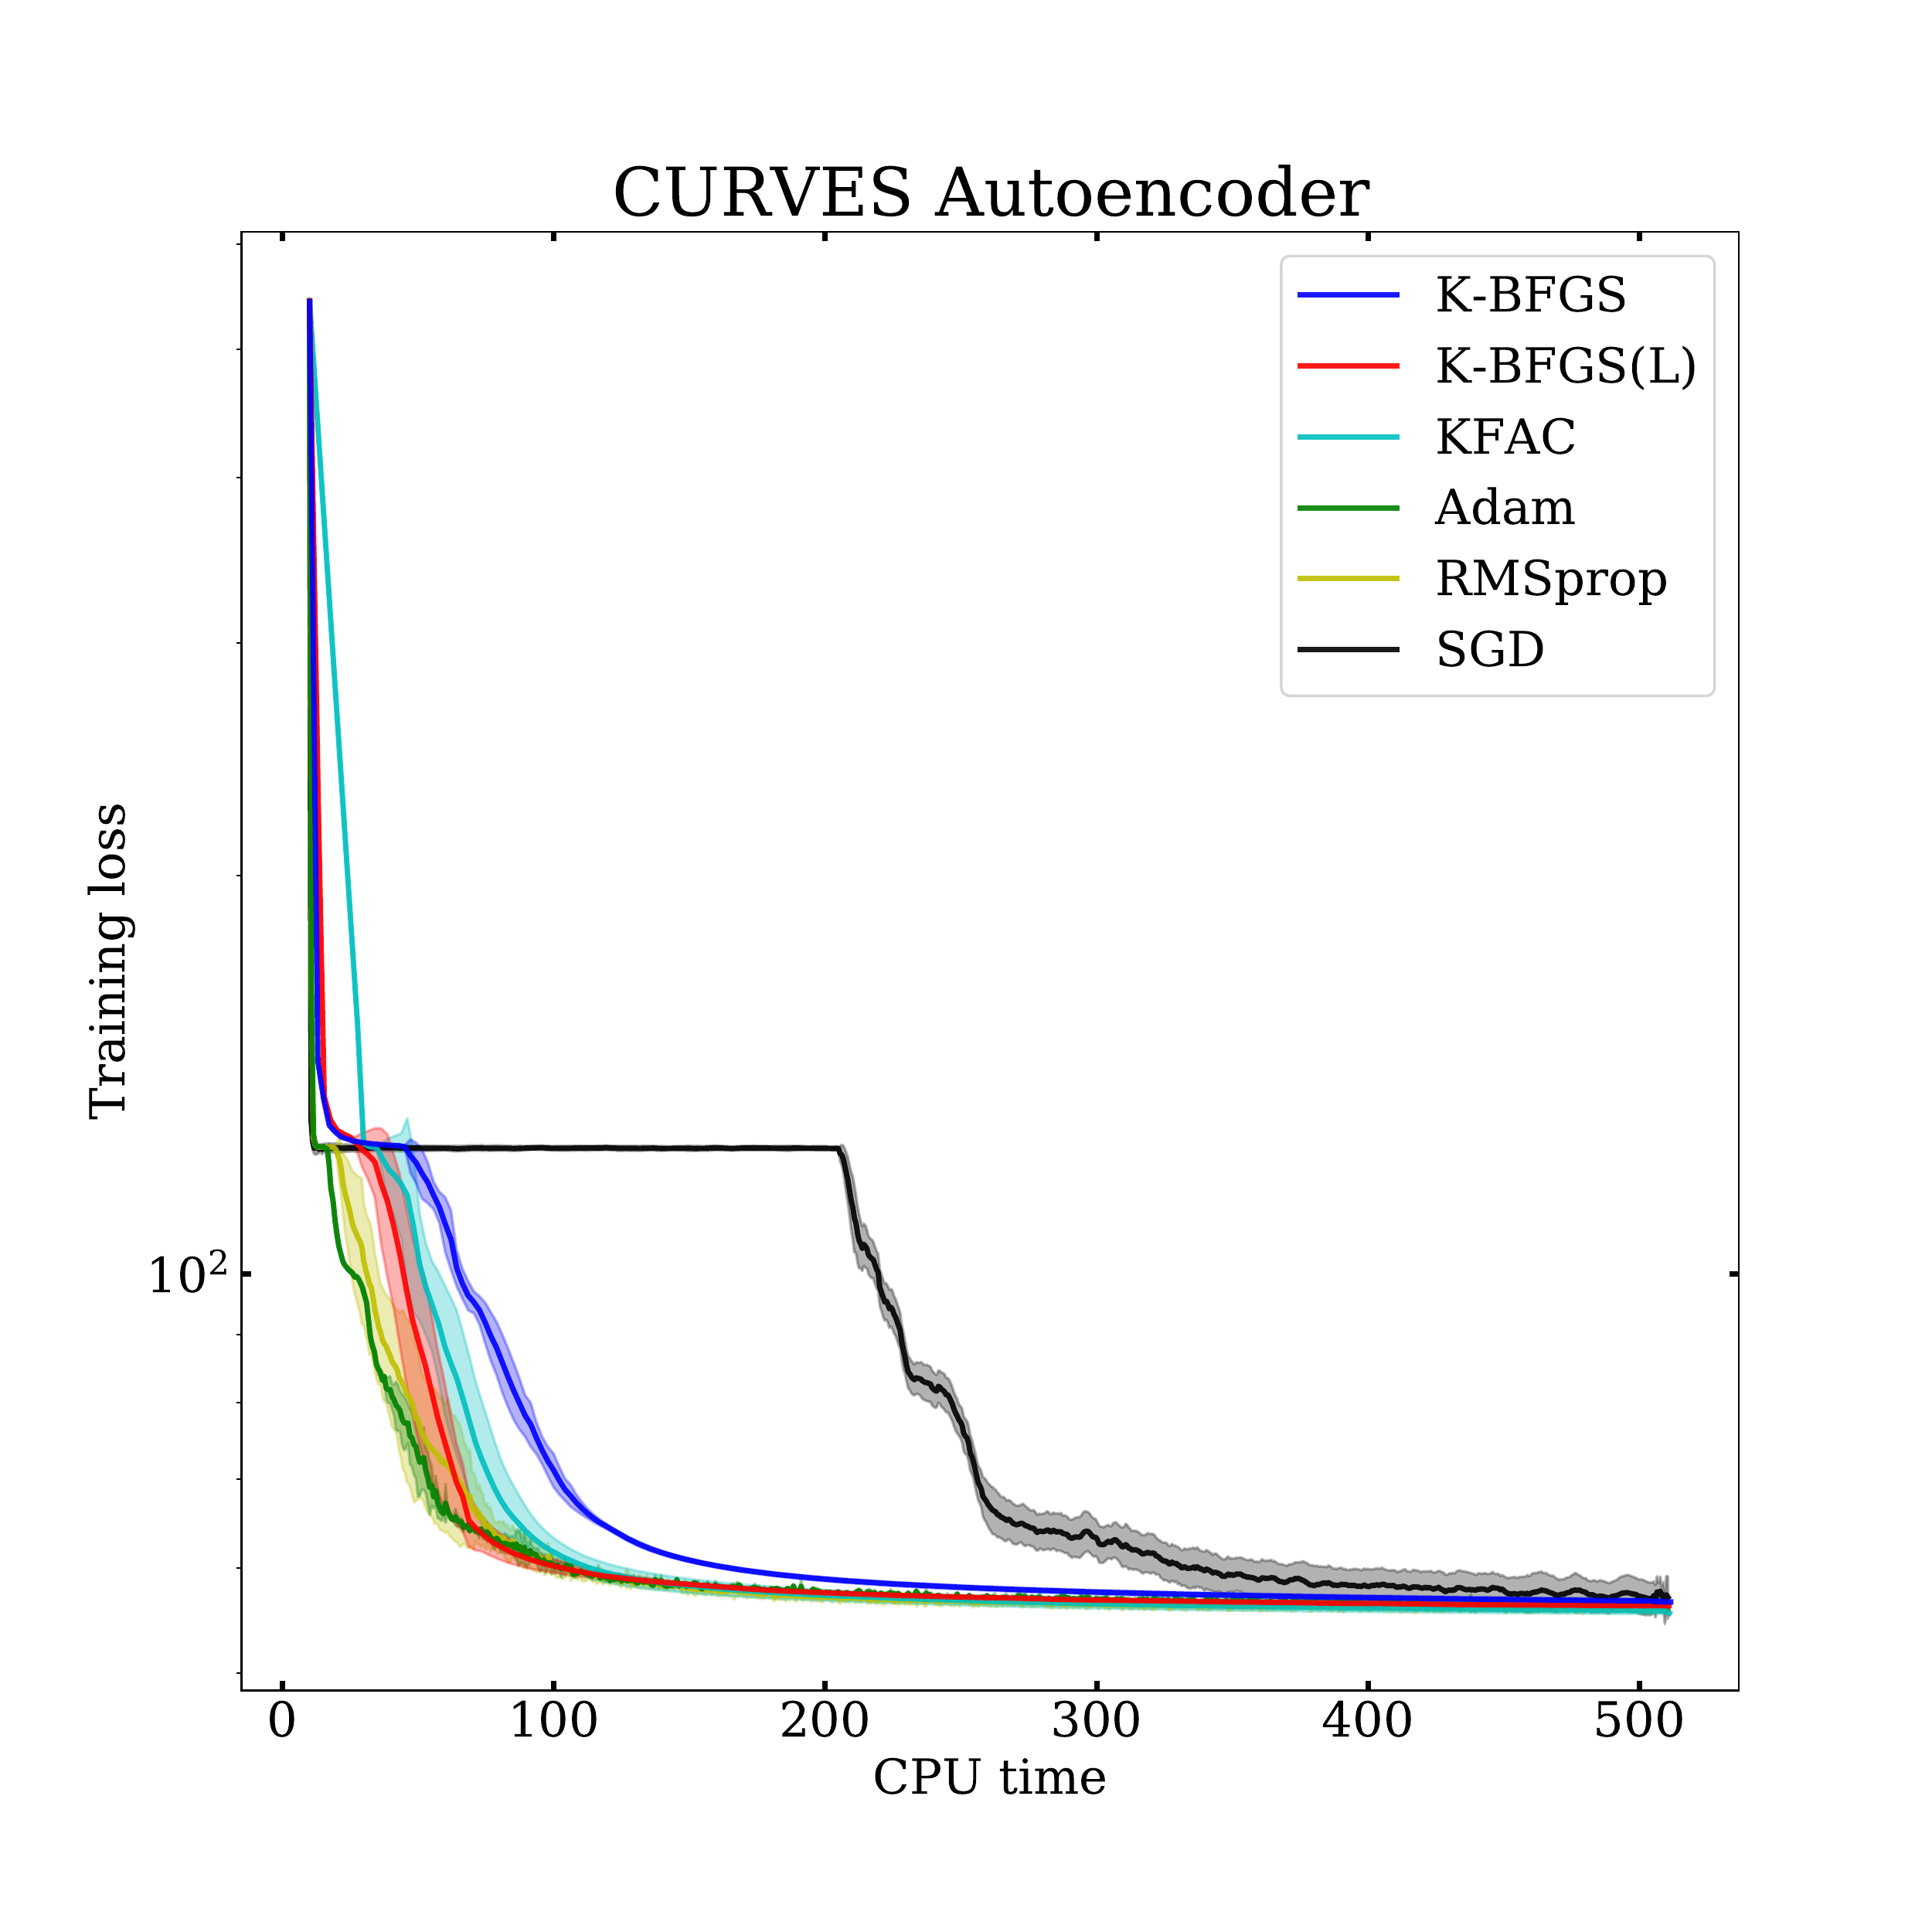}
\end{minipage}

\begin{minipage}{.33\textwidth}
  \centering
  \includegraphics[width=\textwidth]{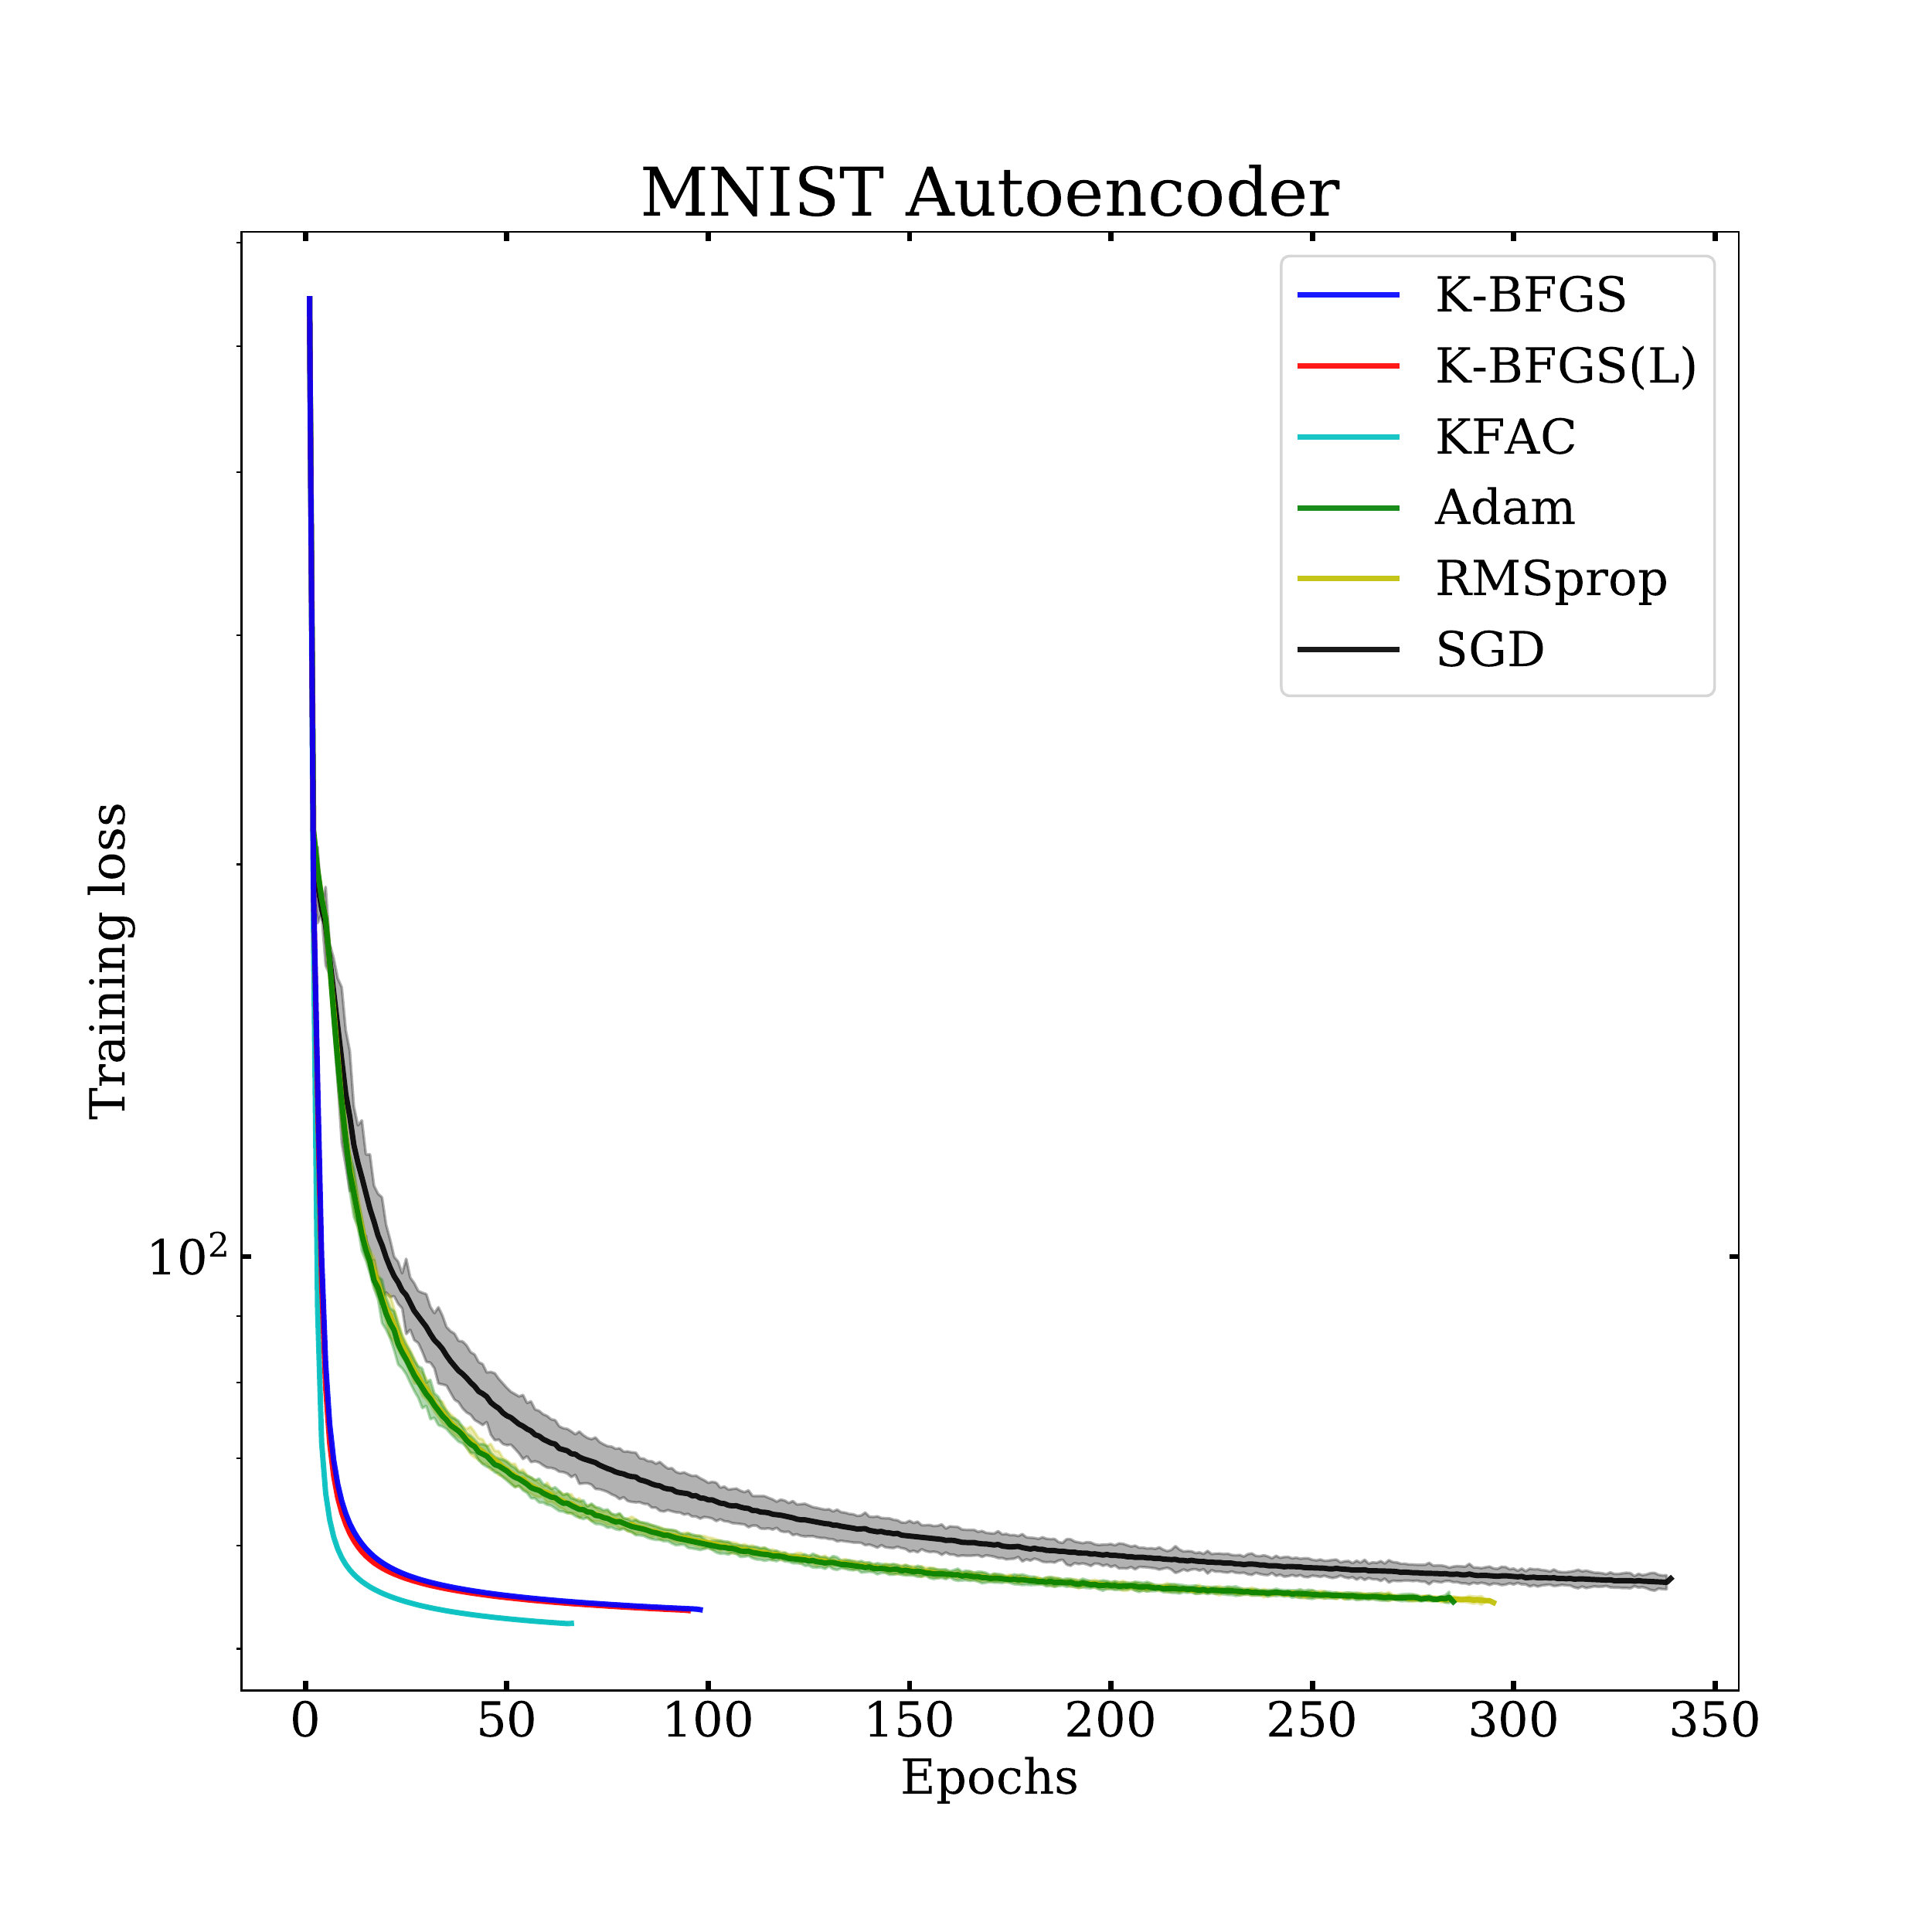}
\end{minipage}%
\begin{minipage}{.33\textwidth}
  \centering
  \includegraphics[width=\textwidth]{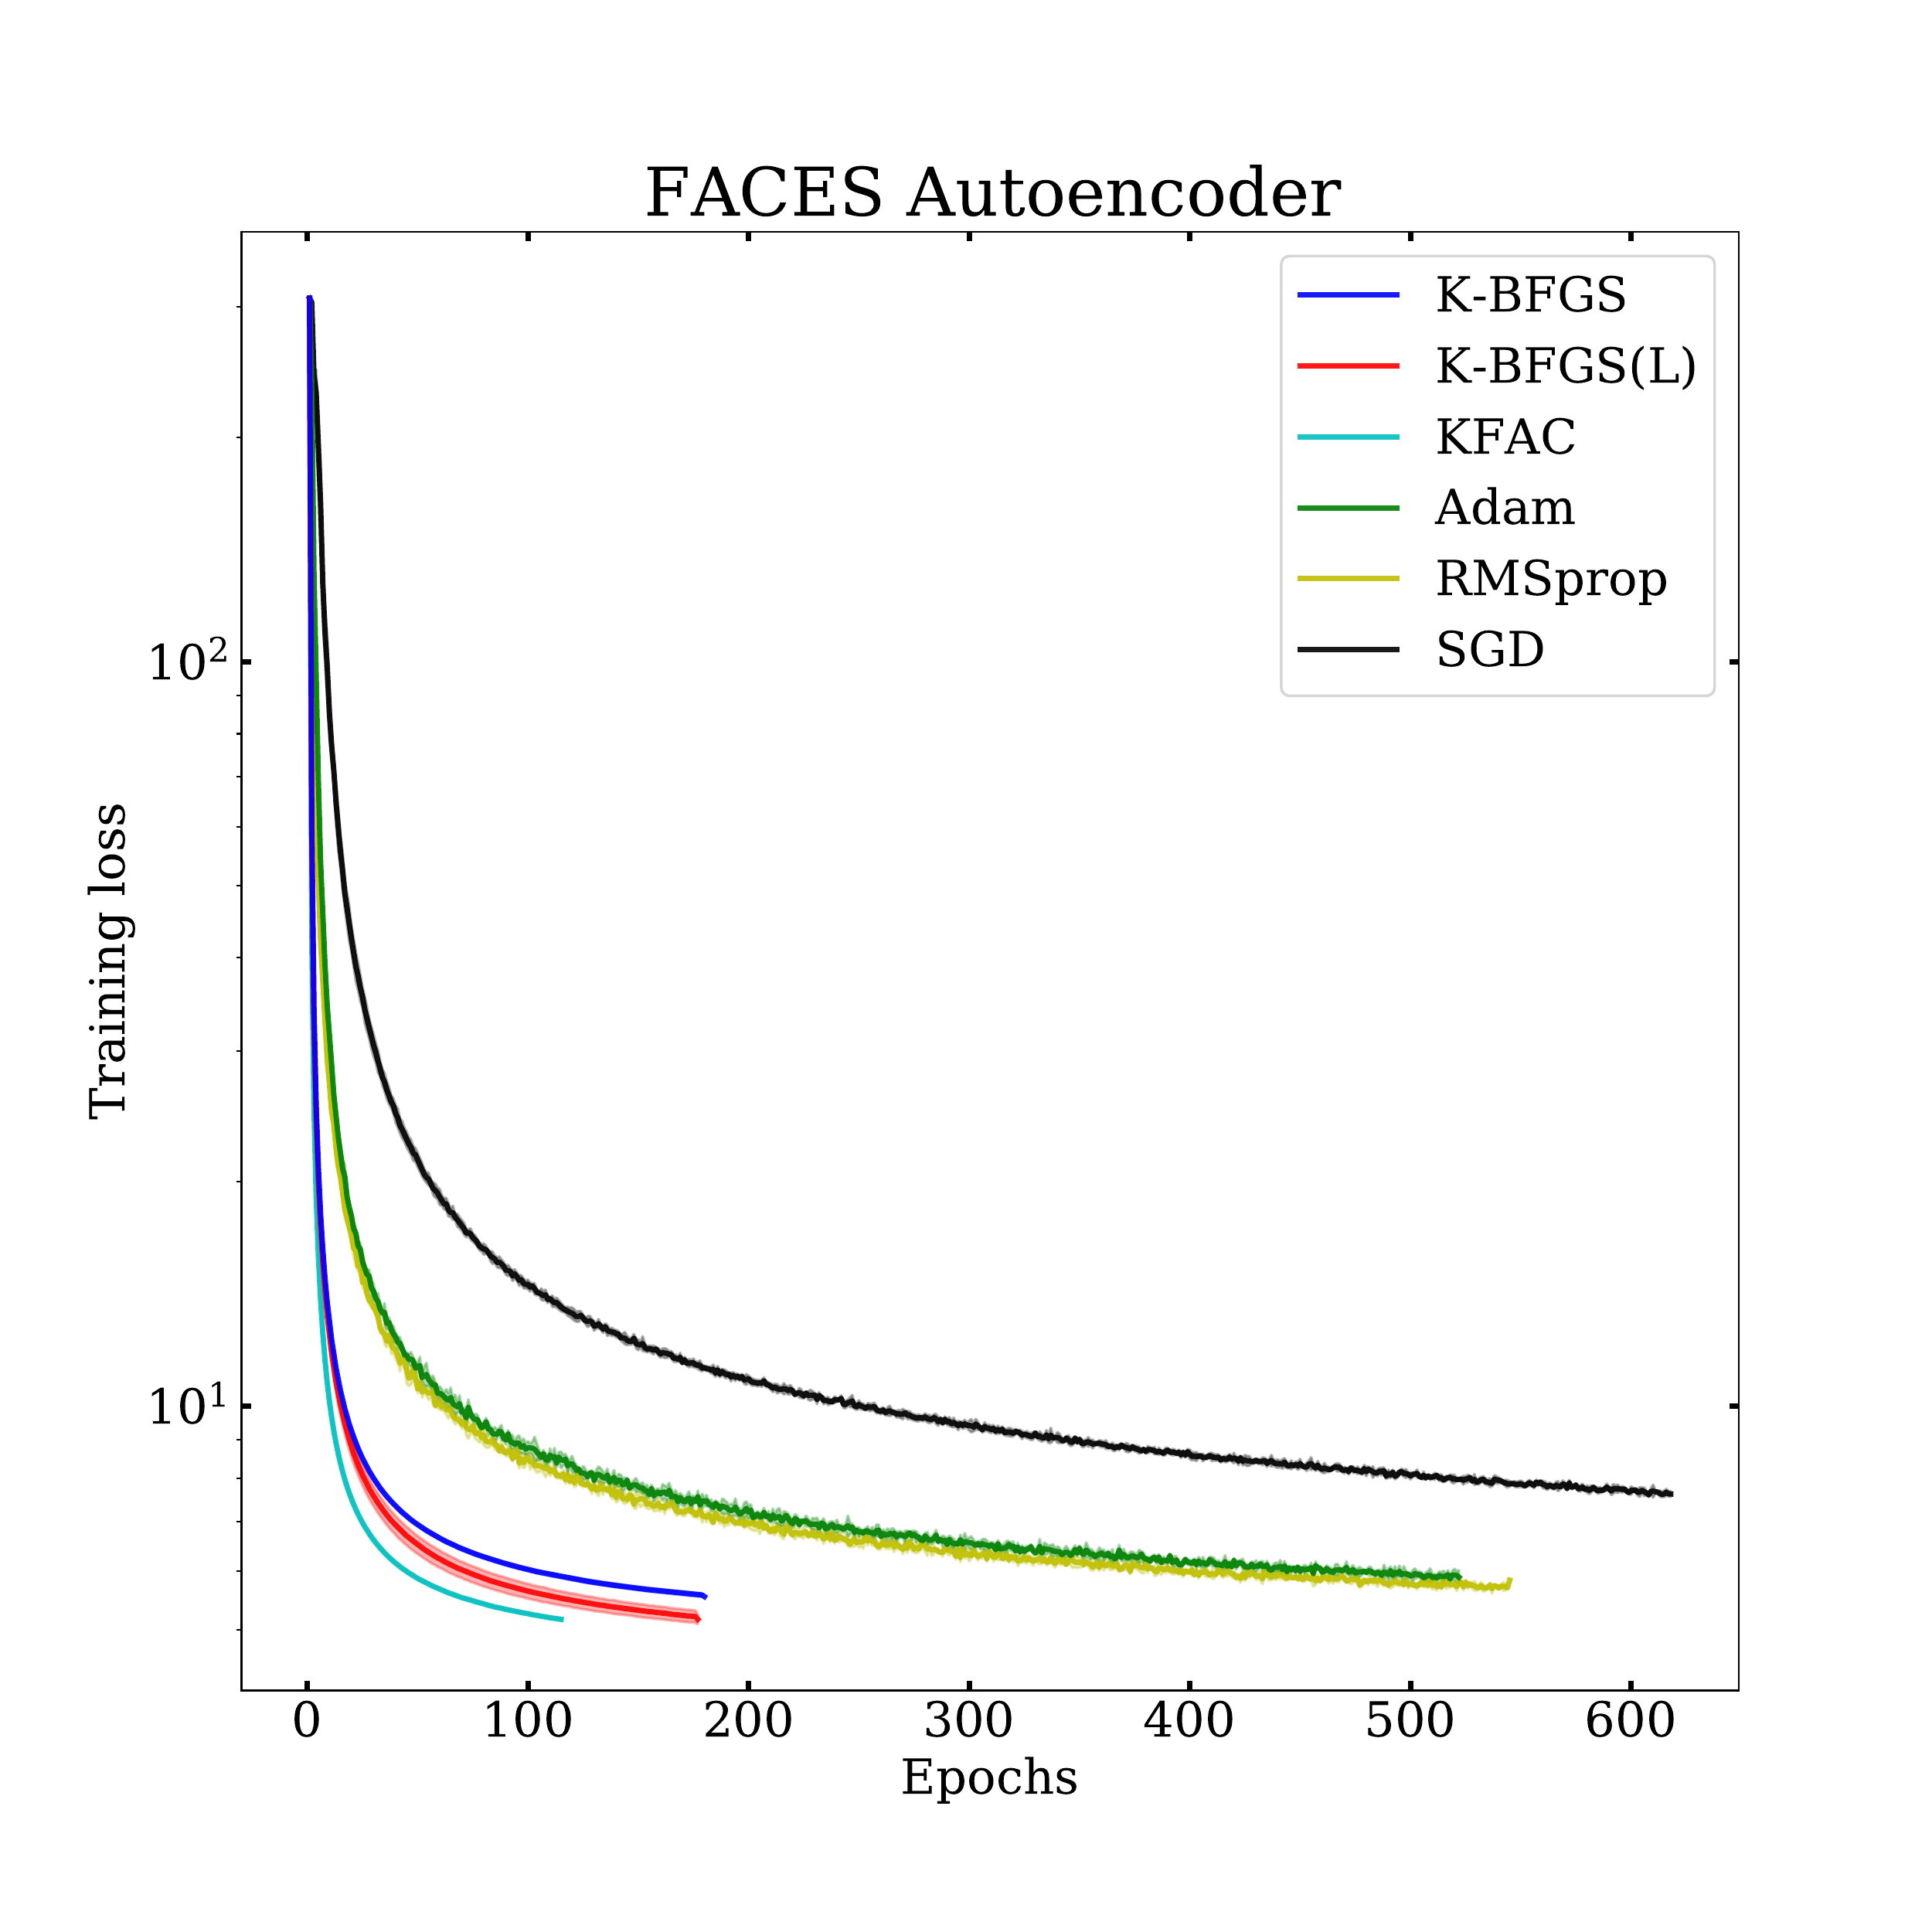}
\end{minipage}%
\begin{minipage}{.33\textwidth}
  \centering
  \includegraphics[width=\textwidth]{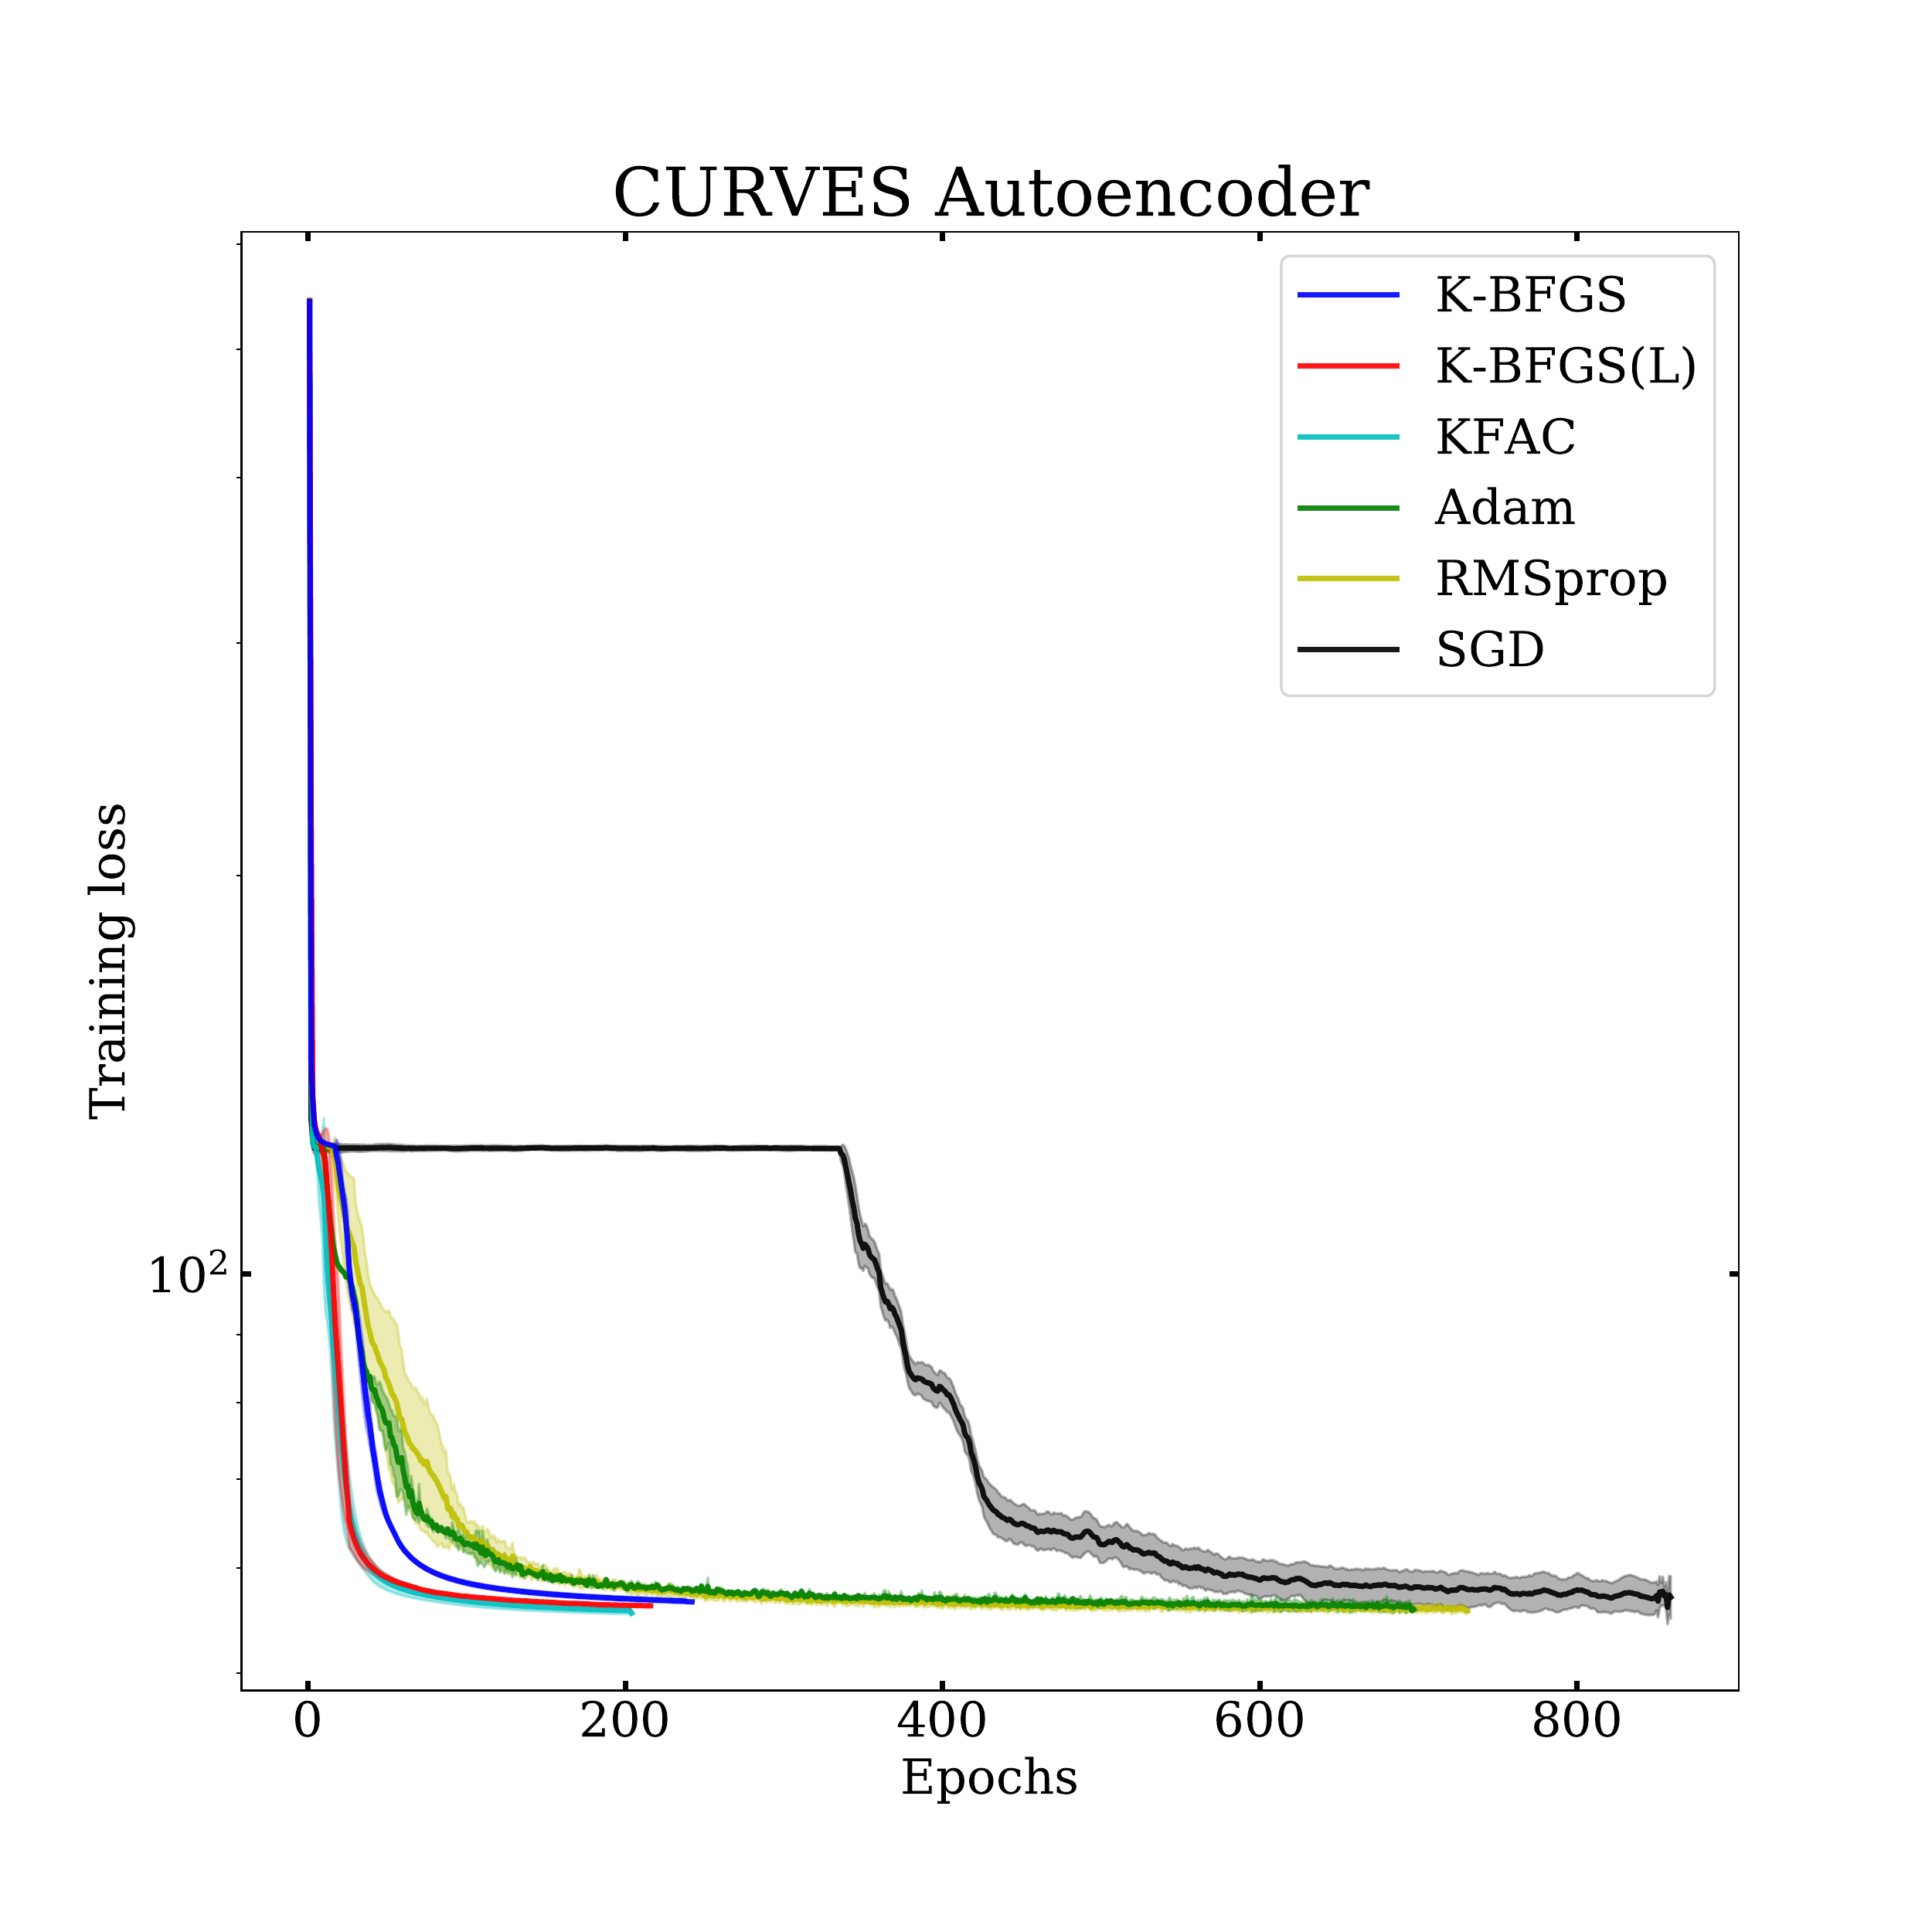}
\end{minipage}

\caption{
Old damping scheme
}
\label{fig_11}
\end{figure}
