# Supplementary material for: Practical Quasi-Newton Methods for Training Deep Neural Networks
Source: arXiv:2006.08877 source file (2021-01-07)
Supplement: Supplementary file 5 [file hessian_action_G.tex]

%\subsection{test}

Following the notation in \cite{botev2017practical}, we first re-state (8) of it:
\begin{align*}
    H_l = B_l W_{l+1}^\top H_{l+1} W_{l+1} B_l + D_l,
\end{align*}
where $l$ is the index of layer. Hence, for a vector $\vs_l$,
\begin{align*}
    H_l \vs_l = B_l W_{l+1}^\top H_{l+1} W_{l+1} B_l \vs_l + D_l \vs_l.
\end{align*}
If we define $\vs_{l+1} = W_{l+1} B_l \vs_l$, we have
\begin{align*}
    H_l \vs_l = B_l W_{l+1}^\top H_{l+1} \vs_{l+1} + D_l \vs_l.
\end{align*}
If we further let $\vy_l = H_l \vs_l$, we have
\begin{align*}
    \vy_l = B_l W_{l+1}^\top \vy_{l+1} + D_l \vs_l.
\end{align*}

Hence, we can get the $(\vs_l, \vy_l)$ pairs for all layers as follows:
\begin{itemize}
    \item Choose an $\vs_1$. 
    
    \item Get all $\vs_l$ by 
    \begin{align*}
        \vs_{l+1} = W_{l+1} B_l \vs_l.
    \end{align*}
    
    \item Compute $\vy_L = H_L \vs_L$. 
    
    \item Get all $\vy_l$ by
    \begin{align*}
        \vy_l = B_l W_{l+1}^\top \vy_{l+1} + D_l \vs_l.
    \end{align*}
\end{itemize}
(It seems to me that) This can be easily paralleled for the mini-batch case. 

% \subsection{}

\subsection{Another concern about K-BFGS}

I always have another concern about K-BFGS, which is kind of a more fundamental issue beyond the various damping schemes. And it is becoming more and more worrying to me as we struggle with the damping part.

Note that in a classical BFGS method, the $(s,y)$ pair is (change in $x$, change in gradient). On the other hand, in K-BFGS, the Hessian (and its inverse $H_g$) we care about is w.r.t the pre-activation $h_l$. Consequently, the $(s_l, y_l)$ pair is (change in $h_l$, change in $dh_l$). ($l$ denotes the index of layer here.)

Currently, we get all $(s_l, y_l)$ pairs ($l=1,...,L$) at one shot, by updating W to be $W^+ = W + p$. Then, a forward and backward pass would give us all (change in $h_l$, change in $dh_l$) all at once. This is a highly efficient way. However, it seems to me that the resulting $(s_l, y_l)$ pairs are questionable.

To see why it is questionable: For a fixed $l$, if we only consider the network after layer $l$, the loss function is determined by $h_l$ and $(W_{l+1}, ..., W_L)$. In other words, we can rewrite the loss function to be $f=f(h_l, W_{l+1}, ..., W_{L})$. The Hessian we care about is the Hessian of $f$ w.r.t $h_l$. Hence, the correct $(s,y)$ pair for $h_l$ should be by changing $h_l$ while keeping $W_{l+1}, ..., W_L$ fixed.

However, recall that in K-BFGS, we get the $(s,y)$ pairs by changing $W$ (i.e. $W_1, ..., W_L$). Changing $W_1, ..., W_l$ gives us the change in $h_l$. But it also makes $W_{l+1}, ..., W_L$ change, which we don't want. As a result, it is hard to say whether the change in $dh_l$ comes from change in $h_l$ or change in $W_{l+1}, ..., W_L$. Thus, the $(s,y)$ pair becomes questionable.

Again, the current way of K-BFGS is purely for the purpose of efficient computation. To verify the above concern, we could try a less efficient way in which we get the $(s, y)$ pairs one layer at a time, which will eliminate the above issue. But, the computational complexity will rise from $O(L)$ to $O(L^2)$.

%If we ignore the computation issue for now, I'm still not sure if this is 
