# Supplementary material for: Practical Quasi-Newton Methods for Training Deep Neural Networks
Source: arXiv:2006.08877 source file (2021-01-07)
Supplement: Supplementary file 6 [file k-bfgs-lm.tex]

This section describes several alternatives about using damping term in K-BFGS. 

\subsection{Sources of damping term}

There are two sources of damping term:
\begin{itemize}
    \item $l_2$ regularization: $\eta$
    
    \item adjustable damping term: $\lambda$
\end{itemize}

The overall damping term that goes into the curvature matrix is $\eta + \lambda$. But there are several differences between them:
\begin{itemize}
    \item $\eta$ is usually added in sake of getting better generalization of the model. $\lambda$ is added for the purposed of controlling how good the quadratic model is. 
    
    \item $\eta$ is usually not adjustable. Typical values of $\eta$ are $0, 10^{-5}, 10^{-3}$. $\lambda$ can be automatically adjusted by Levenberg-Marquardt (LM) approach, or keep fixed. 
    
    \item $\eta$ is included in objective function (i.e. loss function), gradient and curvature. $\lambda$ is included ONLY in curvature. 
\end{itemize}

\subsection{Automatically adjusting \texorpdfstring{$\lambda$}{TEXT}}

%\subsection{Update $\lambda$}

In K-BFGS-LM, we let our approximation to be $(A + \epsilon I_A) \otimes H^{-1}$. Also, we assume that there is a damping term $\lambda$, such that $(A + \epsilon I_A) \otimes H^{-1} \approx A \otimes H^{-1} + \lambda I$. 

To automatically adjust the value of $\lambda$, we follow the practice of Section 4.1 of \cite{martens2010deep}, except that we use a different $q_{\theta}()$ in the definition of $\rho$. More specifically, instead of using the Gauss-Newton matrix, we use the matrix induced by K-BFGS-LM. In other words,
\begin{align*}
    q_\theta(p)
    = f(\theta) + \nabla f(\theta)^\top p + \frac{1}{2} p^\top \left( (A + \epsilon I_A) \otimes H^{-1} \right) p
\end{align*}
Thus, since $p^* = -\left( (A + \epsilon I_A) \otimes H^{-1} \right)^{-1} \nabla f(\theta)$,
\begin{align*}
    q_\theta(p^*) - q_\theta(0)
    = \nabla f(\theta)^\top p^* + \frac{1}{2} (p^*)^\top \left( (A + \epsilon I_A) \otimes H^{-1} \right) p^*
    \\
    = \nabla f(\theta)^\top p^* - \frac{1}{2} (p^*)^\top \nabla f(\theta)
    = \frac{1}{2} \nabla f(\theta)^\top p^*,
\end{align*}
which is very easy to compute since we already have $\nabla f(\theta)$ and $p^*$.

(A side note: we can also use the sub-sampled Hessian matrix, which also should be not too complicated to compute, since we only need Hessian-vector product.)

Algorithm \ref{algo_1} states how we update $\lambda$. It is performs every iteration. Consequently, $f()$ is evaluated using the current mini-batch, $\nabla f(\theta)$ is the stochastic gradient from the current mini-batch. Also note that the choice of boost/drop parameters (i.e. $1.01$ and $1/1.01$) is different the one from \cite{martens2010deep} (i.e. $\frac{3}{2}$ and $\frac{2}{3}$). The value is inspired by \cite{kiros2013training}, as it helps stabilize the change of $\lambda$ in a more stochastic setting. 

\begin{algorithm}
    \caption{Updating $\lambda$}
    \label{algo_1}
    \begin{algorithmic}[1]
    
    \STATE
    $\rho = \frac{f(\theta + p^*) - f(\theta)}{\frac{1}{2} \nabla f(\theta)^\top p^*}$
    
    \IF {$\rho < \frac{1}{4}$}
    \STATE $\lambda = 1.01 \cdot \lambda$
    \ELSIF {$\rho > \frac{3}{4}$}
    \STATE $\lambda = \lambda / 1.01$
    \ENDIF

    \end{algorithmic}
\end{algorithm}

This section explains how to automatically adjust the $\epsilon$ in K-BFGS by a Levenberg-Marquardt (LM) approach. 

Let us consider a single layer, where we (conceptually) assume the Hessian w.r.t. this layer is $B_a \otimes B_g$. In K-BFGS, we further approximates $B_a \otimes B_g$ by $A \otimes H^{-1}$, where $A$ is constantly accumulating information from $a a^\top$ and $H$ is the BFGS matrix which approximates the inverse of $B_g$.

\subsection{From \texorpdfstring{$\lambda$}{TEXT} to \texorpdfstring{$\epsilon$}{TEXT}}

In KFAC, $\lambda$ will be splitted into both $B_a$ and $B_g$ (see Section 6.3 of \cite{martens2015optimizing}). However, in K-BFGS, we'd like to keep the BFGS undamped, but inverting $A$ with a damping term $\epsilon$. Hence, we want
\begin{align*}
    & (A + \epsilon I_A) \otimes H^{-1} \approx A \otimes H^{-1} + \lambda I
    \\
    \Leftrightarrow
    & \epsilon I_A \otimes H^{-1} \approx \lambda I
    \\
    \Leftrightarrow
    & \epsilon H^{-1} \approx \lambda I_H
    \\
    \Leftrightarrow
    & \epsilon I_H \approx \lambda H
    \\
    \Rightarrow
    & \text{tr} \left( \epsilon I_H \right) = \text{tr} \left( \lambda H \right)
    \\
    & \text{(here we go from matrix similarity to matrix trace similarity)}
    \\
    \Leftrightarrow
    & \epsilon d_H = \lambda \cdot \text{tr} \left( H \right)
    \\
    \Leftrightarrow
    & \epsilon = \frac{\lambda \cdot \text{tr} \left( H \right)}{d_H}
\end{align*}
