# Supplementary material for: Practical Quasi-Newton Methods for Training Deep Neural Networks
Source: arXiv:2006.08877 source file (2021-01-07)
Supplement: Supplementary file 7 [file proof_not_used.tex]

To prove the convergence of K-LBFGS, we make the following assumptions.

% \begin{itemize}

% \item
\begin{assumption}
\label{assumption_3}
$f: \R^n\to \R$ is continuously differentiable, and bounded below; 
$f(x) \geq f^{low} > -\infty$, for all $x\in\R^n$. $\nabla f$ is globally Lipschitz continuous with Lipschitz constant $L$; namely for all $x,y\in\R^n$,
    \[
    \|\nabla f(x) - \nabla f(y)\| \le L\|x-y\|.
    \]
\end{assumption}

% \item
% [\textbf{AS.1}] 

%[\textbf{AS.2}] 
\begin{assumption}
\label{assumption_4}
At each iteration $k$, we have
\begin{align}
  a)\quad & \E_{\xi_k}\left[g(x_k,\xi_k)\right]=\nabla f(x_k),\\
  b)\quad & \E_{\xi_k}\left[\|g(x_k,\xi_k)-\nabla f(x_k)\|^2\right]\le \sigma^2, \label{c}
\end{align}
where $\sigma>0$ is the noise level of the gradient estimation, $\xi_k$, $k=1,2,\ldots$, are independent samples, and for a given $k$ the random variable $\xi_k$ is independent of $\{x_j\}_{j=1}^k$.
\end{assumption}

\begin{assumption}
% [\textbf{AS.3}] 
The function $f(x,\xi)$ is twice continuously differentiable with respect to $x$, and there exists a positive constant $\kappa$ such that $\|\nabla_{xx}^2 f(x,\xi)\|\le \kappa$, for any $x,\xi$.
\end{assumption}

\begin{theorem}\label{cvgencetheorem}
Suppose that assumptions {\bf AS.1-4} hold for $\{x_k\}$ generated by Algorithm \ref{klbfgs_2} with batch size $m_k = {m}$ for all $k$. If we choose 
%$\alpha_k$ is specifically chosen as
\begin{align*}
    \alpha_k = \frac{\epsilon^2 \underline{\kappa}}{L (1+\epsilon+\max_l d_l) \bar{\kappa}^2}k^{-\beta}
\end{align*}\label{alpha-spec}
with $\beta\in(0.5,1)$, then after $N$ iterations
\begin{align*}
%\label{conv-rate}
  \frac{1}{N}\sum_{k=1}^N \E[\|\nabla f(x_k)\|^2] \le  \frac{2L(M_f-f^{low}) (1+\epsilon+\max_l d_l)^2 \bar{\kappa}^2}{\epsilon^2\underline{\kappa}^2}N^{\beta-1} + \frac{\sigma^2 }{(1-\beta)m}(N^{-\beta}-N^{-1}).
\end{align*}
%where $N$ denotes the iteration number.
%Moreover, for a given $\epsilon_1 \in(0,1)$, to guarantee that $\frac{1}{N}\sum_{k=1}^N \E[\|\nabla f(x_k)\|^2] < \epsilon_1 $, the number of iterations $N$ needed is at most
%$O\left(\epsilon_1^{-\frac{1}{1-\beta}}\right)$.
\end{theorem}

\clarify{below not finished}

% \addthis{
\begin{proof}
Taking expectation on both sides of (\ref{eq_20}) and summing over $k=1, \ldots, N$ yields

\clarify{$M_f$ has to do with Thm 2.5 in Shiqian's paper}

% \[
\begin{align*}
\frac{1}{2} \underline{\kappa} \sum_{k=1}^{N} \mathbb{E}\left[\left\|\nabla f\left(x_{k}\right)\right\|^{2}\right] 
& \leq \sum_{k=1}^{N} \frac{1}{\alpha_{k}}\left(\mathbb{E}\left[f\left(x_{k}\right)\right]-\mathbb{E}\left[f\left(x_{k+1}\right)\right]\right)+\frac{L \sigma^{2} \bar{\kappa}^{2}}{2 m} \sum_{k=1}^{N} \alpha_{k} \\
&=\frac{1}{\alpha_{1}} f\left(x_{1}\right)+\sum_{k=2}^{N}\left(\frac{1}{\alpha_{k}}-\frac{1}{\alpha_{k-1}}\right) \mathbb{E}\left[f\left(x_{k}\right)\right]
-\frac{\mathbb{E}\left[f\left(x_{N+1}\right)\right]}{\alpha_{N}}+\frac{L \sigma^{2} \bar{\kappa}^{2}}{2 m} \sum_{k=1}^{N} \alpha_{k}
\\
& \leq \frac{M_{f}}{\alpha_{1}}+M_{f} \sum_{k=2}^{N}\left(\frac{1}{\alpha_{k}}-\frac{1}{\alpha_{k-1}}\right)-\frac{f^{l o w}}{\alpha_{N}}+\frac{L \sigma^{2} \bar{\kappa}^{2}}{2 m} \sum_{k=1}^{N} \alpha_{k}
\\
& =\frac{M_{f}-f^{l o w}}{\alpha_{N}}+\frac{L \sigma^{2} \bar{\kappa}^{2}}{2 m} \sum_{k=1}^{N} \alpha_{k}
\\
& \leq \frac{L\left(M_{f}-f^{l o w}\right) \bar{\kappa}^{2}}{\underline{\kappa}} N^{\beta}+\frac{\sigma^{2} \underline{\kappa}}{2(1-\beta) m}\left(N^{1-\beta}-1\right)
\end{align*}
% \]
which results in $(2.23),$ where the second inequality is due to (2.15) and the last inequality is due to $(2.22) .$ Then for a given $\epsilon>0,$ to guarantee that $\frac{1}{N} \sum_{k=1}^{N}$ $\mathbb{E}\left[\left\|\nabla f\left(x_{k}\right)\right\|^{2}\right] \leq \epsilon,$ it suffices to require that
\[
\frac{2 L\left(M_{f}-f^{l o w}\right) \bar{\kappa}^{2}}{\underline{\kappa}^{2}} N^{\beta-1}+\frac{\sigma^{2}}{(1-\beta) m}\left(N^{-\beta}-N^{-1}\right)<\epsilon
\]
since $\beta \in(0.5,1),$ it follows that the number of iterations $N$ needed is at most $O\left(\epsilon^{-\frac{1}{1-\beta}}\right)$

\end{proof}
% }

To simplify notation, let $(s_j, \bar{y}_j)$ denote the pair $(\vs_g^l(j), \bar{\vy}_g^l(j))$ stored by
\deletethis{Algorithm 3}
\addthis{Algorithm \ref{klbfgs_2}}
at iteration $j$, and $H_{k,i}$ denote the $i$-th matrix used to compute the L-BFGS approximation $H_g^l(k)$ by the recursive procedure:\\ 
 (i) compute $H_{k,0}=\gamma_k^{-1} I, \mbox{ where } \gamma_k = \max\left\{
 \frac{y_{k-1}^\top y_{k-1}}{s_{k-1}^\top y_{k-1}} , \delta\right\}$ \\
 %of the inverse Hessian $H_g^l(k)$ at the current iterate $x_k$ and $p$ stored pairs $\{s_j\}$, $\{\bar{y}_j\}$, $j=k-p,\ldots,k-1$, where $p$ is the memory size, the L-BFGS method updates $H_{k,i}$ recursively as
 (ii) For $i=1,\ldots$, compute
$
H_{k,i} = (I-\rho_{j} s_{j} \bar{y}_{j}^\top)H_{k,i-1}(I-\rho_{j} \bar{y}_{j} s_{j}^\top) + \rho_{j} s_{j} s_{j}^\top, \quad j=k-(p-i+1); \, i=1,\ldots,p,
$
where $\rho_{j}=(s_j^\top \bar{y}_j)^{-1}$.

\clarify{need to change the above procedure}

The output $H_{k,p}$ is then used as the estimate of the inverse pre-activation Hessian at $x_k$. We now 
% \deletethis{prove}
{have Lemma \ref{low} showing} that the spectral norm of $H_g^l$ is bounded.

\begin{lemma}
\label{low}
Suppose that {\bf AS.3} holds. Then for every layer $l$,
\begin{enumerate}[label=(\roman*)]
    \item For any  $x,\xi$,
     $\|G_l(x,\xi)\|\le \kappa$, where
     $G_l(x,\xi) := \left( \frac{\partial ^2 f}{\partial h_i^l \partial h_j^l}(x,\xi) \right)_{1\leq i,j\leq d_l}$ is the pre-activation Hessian and $d_l$ is the output size at layer $l$.

    \item Moreover, there exist positive constants 
    % \deletethis{$\underline{\kappa}$ and $\bar{\kappa}$}
    {$\underline{\kappa}_g$ and $\bar{\kappa}_g$} , such that \deletethis{at iteration $k$}.
    \begin{align}
    \underline{\kappa}_g I  \preceq  H_g^l(k)  \preceq  \bar{\kappa}_g I \label{eq_110}
    \quad \forall k, l.
    \end{align}
\end{enumerate}
\end{lemma}

\clarify{need to update the proof}

% {\bf Proof of Lemma \ref{low}:}
\begin{proof}
(i) Let $x,\xi$ be associated with a random single data-point draw and a layer $l$. Then as shown in \cite{botev2017practical}, \cite{martens2015optimizing},
corresponding to layer $l$ the diagonal block of $\nabla_{xx}^2 f(x,\xi)$ is given by

\[
    \nabla^2 f_l(x, \xi) = (\bar{\va}_{l-1} \bar{\va}_{l-1}^\top) \otimes G_l(x, \xi),
\]
Let $z \in \R^{d_l}$ and 

% \clarify{Don: seems like xv is not a defined command. Can you tell me what xv is for so that I can add it in the header? -Yi}

$\vx_l^T =( 0_{d_1}^T, \ldots,(\bar{e}_{l-1} \otimes z)^T,\ldots,  0_{d_L}^T)$,
where $\bar{e}_{l-1} = (0_{dim(\va_{l-1}^T)}, 1)$. Since $\bar{\va}_{l-1}^T = \homovec{\va_{l-1}^T}$, we have $\langle \bar{e}_{l-1}, \bar{\va}_{l-1} \rangle^2 = 1$. Hence,
\begin{align*}
    \vx_l^\top \nabla_{xx}^2 f(x,\xi) \vx_l
    & = (\bar{e}_{l-1}^\top \otimes z^\top) ((\bar{\va}_{l-1} \bar{\va}_{l-1}^\top) \otimes G_l(x, \xi)) (\bar{e}_{l-1} \otimes z) = \langle \bar{e}_{l-1}, \bar{\va}_{l-1} \rangle^2 z^T G_l(x, \xi) z, 
    \\
    -\kappa   \|z \|^2
    & = -\kappa \|\vx_l\|^2 \leq \vx_l^\top \nabla_{xx}^2 f(x,\xi) \vx_l = z^T G_l(x, \xi) z \leq \kappa \|\vx_l\|^2 = \kappa   \|z \|^2.
\end{align*}
It is easy to see that  when one is working with a mini-batch,the above bounds on the pre-activation Hessian  can be used to obtain 
$$
-\kappa \|z \|^2 \leq z^T G_l(x, \xi) z \leq \kappa \|z \|^2
$$

(ii) It can be shown that $H_{k,i}\succ 0$, $i=1,\ldots,p$ since with the previous choices of $(s_j, \bar{y}_j)$, the damping enforced $(s_j^\top \bar{y}_j) \geq \mu s_j \gamma_j^{-1} s_j > 0$. 
To prove that $H_{k,p} \succeq  \underline{\kappa} I$, we prove that $H_{k,p}=B_{k,p}^{-1} \preceq \frac{1}{ \underline{\kappa}} $ 
where $B_{k,p}$ can be computed recursively as

$$
B_{k,i} = B_{k,i-1} + \frac{\bar{y}_j\bar{y}_j^\top}{s_j^\top \bar{y}_j} - \frac{B_{k,i-1}s_j s_j^\top B_{k,i-1}}{s_j^\top B_{k,i-1}s_j}, \quad j=k-(p-i+1);i=1,\ldots,p,
$$
starting from $B_{k,0}=H_{k,0}^{-1}=\gamma_k I$.
Since $B_{k,0}\succ0$, We also have $B_{k,i}\succ0$ for $i=1,\ldots,p$. 
Moreover, it is easily verified that
\[
\|B_{k,i}\| \le \left\|B_{k,i-1} - \frac{B_{k,i-1}s_j s_j^\top B_{k,i-1}}{s_j^\top B_{k,i-1}s_j}\right\| + \left\|\frac{\bar{y}_j\bar{y}_j^\top}{s_j^\top \bar{y}_j}\right\| \leq
\|B_{k,i-1}\| + \left\|\frac{\bar{y}_j\bar{y}_j^\top}{s_j^\top \bar{y}_j}\right\| =\|B_{k,i-1}\| + \frac{\bar{y}_j^\top\bar{y}_j}{s_j^\top \bar{y}_j}.
\]

From the definition of $\bar{y}_j$ in Algorithm 3 and the facts that $s_j^\top \bar{y}_j\ge \mu s_j^\top B_{j+1,0}s_j$ and $B_{j+1,0}=\gamma_{j+1}I$, we have that for any $j=k-1,\ldots,k-p$
\begin{align*}
\frac{\bar{y}_j^\top\bar{y}_j}{s_j^\top \bar{y}_j} \le  \, \frac{\|\theta_j y_j + (1-\theta_j)B_{j+1,0}s_j\|^2}{\mu s_j^\top B_{j+1,0}s_j} 
=   \, \theta_j^2\frac{y_j^\top y_j}{\mu \gamma_{j+1}s_j^\top s_j} + 2\theta_j(1-\theta_j)\frac{y_j^\top s_j}{ \mu s_j^\top s_j} + (1-\theta_j)^2 \frac{\gamma_{j+1}}{\mu}. \label{proof-lemma-low-1}
\end{align*}

To simplify the proof, we consider an idealistic version of Algorithm \ref{klbfgs_2} where the steps in the $h_l$ and  $h_k, k \neq l$ spaces can be chosen independently. It is possible to do this, but it would lead to an impractical algorithm. Since
 $\mathcal{D} \vh_l(j+1,\xi_{j,l})-\mathcal{D} \vh_l(j,\xi_{j,l})=\int_0^1\frac{d\mathcal{D} \vh_l}{dt}(h_l(j)+ts_j,\xi_{j,l})dt = \int_0^1\nabla_{hh}^2 f(h_l(j)+ts_j,\xi_{j,l})s_jdt$
we have:
\[
y_j = \frac{\sum_{l=1}^{m_j}\mathcal{D} \vh_l(j+1,\xi_{j,l})-\mathcal{D} \vh_l(j,\xi_{j,l})}{m_j} = \frac{1}{m_j}\left(\sum_{l=1}^{m_j}\overline{\nabla^2_{hh} f}(h_l(j),\xi_{j,l},s_j)\right)s_j,
\]
where $\overline{\nabla^2_{hh} f}(h_l(j),\xi_{j,l},s_j) = \int_0^1\nabla_{hh}^2f(h_l(j)+ts_j,\xi_{j,l})dt$. Therefore, for any $j=k-1,\ldots,k-p$, from the facts that $0<\theta_j\le1$ and $\delta\le\gamma_{j+1} \le\kappa+\delta$, and (i) it follows that
\begin{align*}
\frac{\bar{y}_j^\top\bar{y}_j}{s_j^\top \bar{y}_j} &\le \frac{\theta_j^2\kappa^2}{\mu\gamma_{j+1}} + \frac{2}{\mu}\theta_j(1-\theta_j)\kappa + \frac{1}{\mu}(1-\theta_j)^2\gamma_{j+1} \\
&\le \frac{\theta_j^2\kappa^2}{\mu \delta} + \frac{1}{\mu}[(1-\theta_j^2)\kappa + (1-\theta_j)^2\delta] %\notag\\
\le \frac{1}{\mu}(\frac{\kappa^2}{\delta} + \kappa+\delta). 
\end{align*}
Therefore:
$
\|B_{k,i}\|\le \|B_{k,i-1}\| + \frac{1}{\mu}(\frac{\kappa^2}{\delta} + \kappa+\delta).
$
and by induction, we have that
\begin{align}
\|B_k\|=\|B_{k,p}\| \le \, \|B_{k,0}\| + \frac{p}{\mu}\left(\frac{\kappa^2}{\delta} + \kappa+\delta\right)
\le \, \frac{p\kappa^2}{\mu \delta} +(\frac{p}{\mu}+1)(\kappa+\delta) \equiv\frac{1}{\underline{\kappa}}. \label{eq_111}
\end{align}

We therefore obtain a lower bound on $H_g^l (k)$. To obtain an upper bound
using same notation as in \citep{wang2017stochastic}, let $H=H_{k,i-1}$, $H^+=H_{k,i}$, $s=s_j$, $\bar{y}=\bar{y}_j$, $\rho=
%s_j^\top\bar{y}_j)^{-1}=
(s^\top\bar{y})^{-1}$, we write the BFGS update as:
\[H^+ = H -\rho(H\bar{y}s^\top+s\bar{y}^\top H) + \rho ss^\top + \rho^2(\bar{y}^\top H \bar{y})ss^\top.\]
Using the facts that $\|uv^\top\|=\|u\|\cdot\|v\|$ for any vectors $u$ and $v$, $\rho s^\top s = \rho\|s\|^2 = \frac{s^\top s}{s^\top\bar{y}}\leq \frac{1}{\mu \delta}$, and $\frac{\|\bar{y}\|^2}{s^\top\bar{y}}\leq \left(\frac{\kappa^2}{\mu \delta}+\kappa+\delta\right)<\frac{1}{\mu \delta}(\kappa+\delta)^2$, which follows from previous results. We have that
\[\|H^+\|\leq \|H\| + \frac{2\|H\|\cdot\|\bar{y}\|\cdot\|s\|}{s^\top\bar{y}}+\frac{s^\top s}{s^\top\bar{y}}+\frac{s^\top s}{s^\top\bar{y}}\cdot\frac{\|H\|\cdot\|\bar{y}\|^2}{s^\top\bar{y}}.\]
Noting that $\frac{\|\bar{y}\|\|s\|}{s^\top\bar{y}}=\left[\frac{\|\bar{y}\|^2}{s^\top\bar{y}}\cdot\frac{\|s\|^2}{s^\top\bar{y}}\right]^{1/2}$, and defining 
$\beta = 1+\frac{\kappa+\delta}{\mu \delta}$,
it follows that
\begin{align*}\|H^+\|\leq \, \left(1+\frac{2}{\mu \delta}(\kappa+\delta)+\left(\frac{1}{\mu \delta}(\kappa+\delta)\right)^2\right)\|H\|+\frac{1}{\mu \delta}   =   \,
\beta^ \|H\| 
%(1+\frac{\kappa+\delta}{\mu \delta})^2\|H\|
+\frac{1}{\mu \delta},\end{align*}
%Let $\beta = \frac{\kappa+(\mu+1) \delta}{\mu \delta}$. 
%By induction we obtain:
which by induction yields
 \begin{align}
\|H_g^l (k)\| \leq \left(\frac{\beta^{2p}-1}{\beta^{2}-1}\right)\frac{1}{\mu \delta} + \frac{\beta^{2p}}{\delta} = \bar{\kappa} \label{eq_112}
 \end{align}
Hence, the bounds in (\ref{eq_110}) follow from (\ref{eq_111}) and (\ref{eq_112}).
%Therefore, we get:
%\[
%\underline{\kappa} \leq \|H_g^l (k)\| \leq \bar{\kappa}
%\]
\end{proof}

\clarify{this is also eq 13}

\begin{align}
    \sum_{k=1}^{+\infty} \alpha_{k}=+\infty, \quad \sum_{k=1}^{+\infty} \alpha_{k}^{2}<+\infty
    % \label{eq_13}
    \label{eq_25}
\end{align}

\begin{align}
\mathbb{E}\left[H_{k} g_{k} | \xi_{[k-1]}\right]=H_{k} \nabla f\left(x_{k}\right)
\label{eq_16}
\end{align}

\begin{align}
\mathbb{E}\left[g_{k} | x_{k}\right]=\nabla f\left(x_{k}\right), \quad \mathbb{E}\left[\left\|g_{k}-\nabla f\left(x_{k}\right)\right\|^{2} | x_{k}\right] \leq \frac{\sigma^{2}}{m_{k}}
\label{eq_17}
\end{align}

We have Lemma \ref{lemma_1}.
\begin{lemma}
\label{lemma_1}
(Analogous to Lemma 2.2 in \citep{wang2017stochastic})

Suppose that $\left\{x_{k}\right\}$ is generated by Algorithm \ref{klbfgs_2} and assumptions AS.1-AS.4 hold. Further assume that (\ref{eq_25}) holds, and $\alpha_{k} \leq \frac{\kappa}{L \bar{\kappa}^{2}}$ for all $k .$ (Note that this can be satisfied if $\alpha_{k}$ is non-increasing and the initial step size $\alpha_{1} \leq \frac{\kappa}{L \bar{\kappa}^{2}} .$ ) Then the following inequality holds:
\begin{align}
\mathbb{E}\left[f\left(x_{k+1}\right) | x_{k}\right] \leq f\left(x_{k}\right)-\frac{1}{2} \alpha_{k} \underline{\kappa}\left\|\nabla f\left(x_{k}\right)\right\|^{2}+\frac{L \sigma^{2} \bar{\kappa}^{2}}{2 m_{k}} \alpha_{k}^{2} \quad \forall k \geq 1
\label{eq_20}
\end{align}
where the conditional expectation is taken with respect to $\xi_{k}$

\end{lemma}

% {\bf Proof of Lemma \ref{lemma_1}}:

% \addthis{
\begin{proof}

Define $\delta_{k}=g_{k}-\nabla f\left(x_{k}\right) .$ From Lemma \ref{lemma_2} and assumptions AS.\ref{assumption_3} we have
\begin{align}
f\left(x_{k+1}\right) 
& \leq f\left(x_{k}\right)+\left\langle\nabla f\left(x_{k}\right), x_{k+1}-x_{k}\right\rangle+\frac{L}{2}\left\|x_{k+1}-x_{k}\right\|^{2}
& \text{(AS.\ref{assumption_3})}
\nonumber
\\
&=f\left(x_{k}\right)-\alpha_{k}\left\langle\nabla f\left(x_{k}\right), H_{k} g_{k}\right\rangle+\frac{L}{2} \alpha_{k}^{2}\left\|H_{k} g_{k}\right\|^{2}
& \text{(Lemma \ref{lemma_2})}
\nonumber
\\
& \leq f\left(x_{k}\right)-\alpha_{k}\left\langle\nabla f\left(x_{k}\right), H_{k} \nabla f\left(x_{k}\right)\right\rangle-\alpha_{k}\left\langle\nabla f\left(x_{k}\right), H_{k} \delta_{k}\right\rangle+\frac{L}{2} \alpha_{k}^{2} \bar{\kappa}^{2}\left\|g_{k}\right\|^{2}
& \text{(Lemma \ref{lemma_2})}
\label{eq_15}
\end{align}

Taking expectation with respect to $\xi_{k}$ on both sides of (\ref{eq_15}) conditioned on $x_{k},$ we obtain
\begin{align}
\mathbb{E}\left[f\left(x_{k+1}\right) | x_{k}\right] \leq f\left(x_{k}\right)-\alpha_{k}\left\langle\nabla f\left(x_{k}\right), H_{k} \nabla f\left(x_{k}\right)\right\rangle+\frac{L}{2} \alpha_{k}^{2} \bar{\kappa}^{2} \mathbb{E}\left[\left\|g_{k}\right\|^{2} | x_{k}\right]
& \text{(AS.\ref{assumption_4})}
\label{eq_18}
\end{align}
where we used (\ref{eq_16}) and the fact that $\mathbb{E}\left[\delta_{k} | x_{k}\right]=0 .$ From (\ref{eq_17}) and $\mathbb{E}\left[\delta_{k} | x_{k}\right]=0,$ it follows that
\[
\begin{aligned}
\mathbb{E}\left[\left\|g_{k}\right\|^{2} | x_{k}\right] &=\mathbb{E}\left[\left\|g_{k}-\nabla f\left(x_{k}\right)+\nabla f\left(x_{k}\right)\right\|^{2} | x_{k}\right] \\
&=\mathbb{E}\left[\left\|\nabla f\left(x_{k}\right)\right\|^{2} | x_{k}\right]+\mathbb{E}\left[\left\|g_{k}-\nabla f\left(x_{k}\right)\right\|^{2} | x_{k}\right]+2 \mathbb{E}\left[\left\langle\delta_{k}, \nabla f\left(x_{k}\right)\right\rangle | x_{k}\right] \\
&=\left\|\nabla f\left(x_{k}\right)\right\|^{2}+\mathbb{E}\left[\left\|g_{k}-\nabla f\left(x_{k}\right)\right\|^{2} | x_{k}\right] \leq\left\|\nabla f\left(x_{k}\right)\right\|^{2}+\sigma^{2} / m_{k}
\end{aligned}
\]
which together with (\ref{eq_18}) and Lemma \ref{lemma_2} yields that
\begin{align}
\mathbb{E}\left[f\left(x_{k+1}\right) | x_{k}\right] \leq f\left(x_{k}\right)-\left(\alpha_{k} \underline{\kappa}-\frac{L}{2} \alpha_{k}^{2} \bar{\kappa}^{2}\right)\left\|\nabla f\left(x_{k}\right)\right\|^{2}+\frac{L \sigma^{2} \bar{\kappa}^{2}}{2 m_{k}} \alpha_{k}^{2}
\label{eq_19}
\end{align}
Then (\ref{eq_19}) combined with the assumption $\alpha_{k} \leq \frac{\kappa}{L \bar{\kappa}^{2}}$ implies (\ref{eq_20}). 

\end{proof}
