# Supplementary material for: Practical Quasi-Newton Methods for Training Deep Neural Networks
Source: arXiv:2006.08877 source file (2021-01-07)
Supplement: Supplementary file 8 [file another_DD.tex]

% \subsection{Double Damping}

% \clarify{need a new name for this section}

Our double damping, Algorithm \ref{algo_DD} is below.

\begin{algorithm}
    \caption{Double damping}
    \label{algo_DD}
%     %\label{feedforward}
    \begin{algorithmic}[1]
    
%     \REQUIRE $\vs$, $\vy$
%     \ENSURE $\tilde{\vs}$, $\tilde{\vy}$
    
%     \COMMENT{Powell's damping on $H$ - other variants could be used, e.g., Powell's modified damping on $H$}

    \STATE $\sigma \equiv \max\{\vy^\top H \vy, \vs^\top \vs\}$

    \IF
    {
    % \deletethis{$\vs^\top \vy \geq \alpha \sigma$}
    {$\vs^\top \vy \geq \mu \sigma$}
    }
    \STATE $\tilde{\vs} = \vs, \; \tilde{\vy} = \vy$

    \ELSE   
    
    \IF{
    % \deletethis{$\sigma =\vy^\top H \vy \; {\rm and} \; \vs^\top \vy < \alpha \sigma$}
    {
    $\sigma =\vy^\top H \vy \; {\rm and} \; \vs^\top \vy < \mu \sigma$
    }
    }
  
    \STATE
    % \deletethis{$\theta_1 = \frac{(1-\alpha) \vy^\top H \vy}{\vy^\top H \vy - \vs^\top \vy}$}
    {$\theta_1 = \frac{(1-\mu) \vy^\top H \vy}{\vy^\top H \vy - \vs^\top \vy}$}
    
    \STATE $\tilde{\vs} = \theta_1 \vs + (1-\theta_1) H \vy, \;  \tilde{\vy} = \vy $
    \ENDIF

    \IF
    {
    % \deletethis{$\sigma =\vs^\top \vs  \; {\rm and} \;  \vs^\top \vy <  \alpha \sigma$}
    {$\sigma =\vs^\top \vs  \; {\rm and} \;  \vs^\top \vy <  \mu \sigma$}
    }

        \STATE
        % \deletethis{$\theta_2 = \frac{(1-\alpha) \vs^\top \vs}{\vs^\top \vs - \vs^\top \vy}$}
        {$\theta_2 = \frac{(1-\mu) \vs^\top \vs}{\vs^\top \vs - \vs^\top \vy}$} 
        
    \STATE $\tilde{\vy} = \theta_2 \vy + (1-\theta_2) \vs, \; \tilde{\vs} = \vs$
    \ENDIF
    \ENDIF
    
%     \RETURN $\tilde{s}$, $\tilde{y}$
    
    \end{algorithmic}
\end{algorithm}
