# Supplementary material for: Practical Quasi-Newton Methods for Training Deep Neural Networks
Source: arXiv:2006.08877 source file (2021-01-07)
Supplement: Supplementary file 9 [file combination.tex]

\begin{table}[H]
  \caption{}
  %\label{table_1}
  \centering
  \begin{tabular}{l | l | l | l} 
    \toprule
    if block-diagonal dominant
    & if Kron
    & if BFGS
    & comments
    \\
    %\midrule
    \hline
    block-diagonal
    & Kron
    & BFGS
    & our algorithm
    \\
    \cline{3-4}
    & 
    & Newton
    & something very close to KFAC and Botev
    \\
    \cline{2-4}
    & full
    & BFGS
    & layer-wise BFGS
    \\
    \cline{3-4}
    &
    & Newton
    & layer-wise Newton
    \\
    \hline
    full
    & Kron
    & BFGS
    & seems to be a funny combination
    \\
    &
    & Newton
    \\
    \cline{2-4}
    & full
    & BFGS
    & full BFGS
    \\
    \cline{3-4}
    &
    & Newton
    & full Newton
    \\
    \bottomrule
  \end{tabular}
\end{table}
