# Supplementary material for: Practical Quasi-Newton Methods for Training Deep Neural Networks
Source: arXiv:2006.08877 source file (2021-01-07)
Supplement: Supplementary file 10 [file operation_speed.tex]

%\subsection{In practice}

\begin{figure}[ht]
  \centering
  \includegraphics[width=0.5\textwidth]{figures/inv_vs_mm/inv_vs_mm.pdf}
  \caption{Speed comparison between matrix multiplication, inverse and SVD}
  \label{fig_4}
\end{figure}

In Figure \ref{fig_4}, we empirically compare the speed of matrix multiplication, inverse and SVD, which are used {(although can be amortized)} in major non-diagonal second order algorithms {(e.g. inverse in \cite{martens2015optimizing}) and SVD in \cite{gupta2018shampoo})}. On the other hand, K-BFGS and K-BFGS(L) does not involve either inverse or SVD. In particular, "matrix multiplication" refers to the operation of $A \times B$ where $A, B \in R^{d \times d}$, while "matrix inverse" refers to the operation of inverting $A \in R^{d \times d}$ and "SVD" refers to performing the singular value decomposition of $A \in R^{d \times d}$. 

We can see that, although all operations have a theoretical complexity of \deletethis{$O(d^3)$} \addthis{$O(d^\alpha)$ where $2 < \alpha \le 3$}, the actual speed in practice differs a lot. Moreover, the time for matrix inverse and SVD slows down significantly as $d$ becomes larger. {Last but not least, matrix multiplication in nature is more suitable for parallel computation.}

% \clarify{(add CPU vs GPU)}
